# Supplementary material for: RECLAIM: Cyclic Causal Discovery Amid Measurement Noise
Source: arXiv:2603.20585 source file (2026-03-21)
Supplement: Supplementary file 1 [file appendix.tex]

\appendix
\crefalias{section}{appendix}
\crefalias{subsection}{appendix}

\makeatletter\@addtoreset{example}{section}\makeatother

\makeatletter\@addtoreset{theorem}{section}\makeatother

\makeatletter\@addtoreset{assume}{section}\makeatother

\makeatletter\@addtoreset{lemma}{section}\makeatother

\makeatletter\@addtoreset{definition}{section}\makeatother

\makeatletter\@addtoreset{prop}{section}\makeatother

\makeatletter\@addtoreset{algorithm}{section}\makeatother

{
\Large\bfseries
Appendices
}

\vspace{0.3cm}

The appendices are organized as follows. \Cref{sec:solution-to-sem} discusses the solvability of the SCM considered in the work. \Cref{app:convergence} analyses the convergence of the EM algorithm in RECLAIM. \Cref{app:theoretical-considerations} contains all the proofs. \Cref{app:implementation-details} provides additional details on the implementation of RECLAIM and the baselines. Finally, \cref{app:additional-experiments} provides additional experimental results and training time comparison between RECLAIM and the baselines.

% Section on solvability of the SCM
\section{Solvability of Cyclic SCMs}
\label{sec:solution-to-sem}

Consider the cyclic SCM defined below: 
\begin{equation}\label{app-eq:scm}
    \rvx = f(\rvx) + \rvz. 
\end{equation}
% Need for function contractivity
In general, it is not guaranteed that \cref{app-eq:scm} has solution, this is primarily due to the (potential) presence of cycles in $\gr$. In order to see why this is true, note that, we can view \cref{app-eq:scm} as the unique fixed point (if it exists) to the following discrete time dynamical system:
\begin{equation}
    \label{app-eq:discrete-time-dynamical-system}
    \rvx(t+1) = f\big(\rvx(t)\big) + \rvz,
\end{equation}
where $\rvx(t)$ denotes the value of the random variable $\rvx$ at time $t$. In the following example, we illustrate how the choice of $f$ dictates whether or not \cref{app-eq:discrete-time-dynamical-system} attains a unique fixed point.

\begin{example}\label{example:no-fixed-point}
    Consider $X_1, X_2 \in \R$ given by the following structural equations:
    $$X_1(t+1) = aX_2(t) + Z_1, \quad X_2(t+1) = bX_1(t) + Z_2.$$
    \Cref{app-fig:example-no-fixed-point} shows an illustration of the evolution of trajectories for two different choices of the parameters $(a, b)$. From the right plot we can see that when we set $a=1.2$, and $b=2.3$, the systems is unstable and trajectory diverges. On the other hand, when $a=0.7$ and $b=-0.8$ (left plot), the system is stable and reaches a stationary point. 
\end{example}

To ensure \cref{app-eq:discrete-time-dynamical-system} admits a unique fixed point, we must impose additional restrictions on the causal mechanism $f$. One sufficient condition is to require $f$ to be \emph{contractive}.

\begin{definition}[Contractive function]
    A function $f : \R^d \to \R^d$ is said to be contractive if there exists a constant $L < 1$ such that for all $\vx, \vy \in \R^d$,
    $$\norm{f(\vx) - f(\vy)}_2 \leq L \norm{\vx - \vy}_2.$$
    The constant $L$ is called the Lipschitz constant. 
\end{definition}

When the causal mechanism $f$ is contractive, Banach fixed point theorem gaurantees that \cref{app-eq:discrete-time-dynamical-system} has a unique fixed point~\cite[theorem 9.23]{rudin2021principles}. Consequently, the causal mechanisms considered in this work are restricted to be contractive and neural networks are used to model the causal mechanism in practice. Contractivity is achieved via spectral scaling of the layer weights as described in \cref{sec:latent-likelihood} in the main paper. 

\begin{figure}[t]
\centering
\input{app-figures/example-no-fixed-point}
\caption{Illustration of state evolution for different choice of $a$ and $b$ for the system defined in \cref{example:no-fixed-point}. (Left) Choosing $a = 0.7$ and $b=-0.8$ results in a stable system and the system reaches a fixed point. (Right) Choosing $a = 1.2$ and $b = 2.3$ results in an unstable system and the trajectory diverges. }
\label{app-fig:example-no-fixed-point}
\end{figure}

% Section on convergence analysis of EM algorithm
\section{Convergence of EM algorithm}
\label{app:convergence}

Here, we provide the convergence analysis of RECLAIM's EM-based score maximization algorithm. Let $\mTheta^{(t)} = (\vtheta^{(t)}, \hat{\vphi})$. For ease of notation, we focus on a single interventional experiment $I_k \in \si$. However, the final result would still hold even when we consider the sum of likelihood over all the interventional experiments. Our analysis relies on the convergence of the EM algorithm \citep{wu_em_convergence,Friedman1998TheBS}, with the crux of it relying on establishing that the total log-likelihood of the observed variables either increases or stays the same in each iteration of the algorithm. That is, 
\begin{equation}\label{app-eq:m-step-requirement}
    \sum_{\ell=1}^{n_k} \log p(\vy^{(k, \ell)} \mid \mTheta^{t+1}, I_k) \geq \sum_{\ell=1}^{n_k} \log p(\vy^{(k, \ell)} \mid \mTheta^{t}, I_k)
\end{equation}

To that end, note that 
\begin{align*}
   \sum_{i=1}^{n_k} \log p(\vy^{(k, \ell)} \mid \mTheta, I_k) &= \sum_{i=1}^{n_k} \log p(\vy^{(k, \ell)}, \rvx^{(k, \ell)} \mid \mTheta, I_k) \\
    & \qquad - \sum_{i=1}^{n_k} \log p(\rvx^{(k, \ell)}\mid \vy^{(k, \ell)}, \mTheta, I_k)
\end{align*}
Taking expectation with respect $\rvx^{(k, \ell)}\mid \vy^{(k, \ell)}$ on both side, we get
\begin{align}
    \sum_{i=1}^{n_k} \log p(\vy^{(k, \ell)} \mid \mTheta, I_k) &=\sum_{i=1}^{n_k} \expect_{\rvx^{(k, \ell)}\mid \vy^{(k, \ell)}; \mTheta^{t}} \log p(\vy^{(k, \ell)} \mid \mTheta, I_k)\nonumber\\
    &= \underbrace{\sum_{i=1}^{n_k} \expect_{\rvx^{(k, \ell)}\mid \vy^{(k, \ell)}; \mTheta^{t}}\log p(\vy^{(k, \ell)}, \rvx^{(k, \ell)} \mid \mTheta, I_k)}_{= Q(\vtheta|\vtheta^t)}\nonumber\\
    & \quad -\sum_{i=1}^{n_k} \expect_{\rvx^{(k, \ell)}\mid \vy^{(k, \ell)}; \mTheta^{t}}\log p(\rvx^{(k, \ell)}\mid \vy^{(k, \ell)}, \mTheta, I_k).
    \label{app-eq:convergence-1}
\end{align}
The first term on the RHS in the above equation is nothing but $Q(\vtheta| \vtheta^t)$. This is maximized in the M-step, i.e., $Q(\vtheta| \vtheta^{t+1}) \geq Q(\vtheta| \vtheta^t)$. On the other hand, 
\begin{multline*}
\sum_{i=1}^{n_k} \expect_{\rvx^{(k, \ell)}\mid \vy^{(k, \ell)}; \mTheta^{t}}\log \frac{p(\rvx^{(k, \ell)}\mid \vy^{(k, \ell)}, \mTheta^{t+1}, I_k)}{p(\rvx^{(k, \ell)}\mid \vy^{(k, \ell)}, \mTheta^t, I_k)} = \\
 -D_{KL}\Big(p(\rvx^{(k, \ell)}\mid \vy^{(k, \ell)}, \mTheta^t, I_k)\big\|p(\rvx^{(k, \ell)}\mid \vy^{(k, \ell)}, \mTheta^{t+1}, I_k)\Big) \leq 0.
\end{multline*}
Thus, 
\begin{multline}
    \sum_{i=1}^{n_k} \expect_{\rvx^{(k, \ell)}\mid \vy^{(k, \ell)}; \mTheta^{t}}\log p(\rvx^{(k, \ell)}\mid \vy^{(k, \ell)}, \mTheta^{t+1}, I_k) \\ \leq \sum_{i=1}^{n_k} \expect_{\rvx^{(k, \ell)}\mid \vy^{(k, \ell)}; \mTheta^{t}}\log p(\rvx^{(k, \ell)}\mid \vy^{(k, \ell)}, \mTheta^t, I_k).
    \label{app-eq:convergence-2}
\end{multline}
From combining \cref{app-eq:convergence-1,app-eq:convergence-2}, we can see that at the end of the M-step \cref{app-eq:m-step-requirement} is satisfied. Thus, RECLAIM reaches a stationary point of the optimization objective.

% Section containing the main proofs
\section{Proofs}
\label{app:theoretical-considerations}

All the proofs are contained in this section. Starting with proof of \cref{prop:projection-existence} in \cref{app:prop-projection-existence-proof}. \Cref{app:theorem-full-rank-possible-proof} contains the proof of \cref{theorem:full-rank-possible}. Finally, \cref{app:theorem-consistency-proof} contains the proof for \cref{theorem:consistency}. 

\subsection{Proof of \texorpdfstring{\Cref{prop:projection-existence}}{Proposition 3}}

\label{app:prop-projection-existence-proof}

\begin{proof}
    The claim of the proposition is equivalent to the following statement: 
    $$\mathcal{N}(\mA_{-i}^\top) \not\subset \veca_i^\perp.$$
    Since $\rank(\mA) = d$, the vector $\veca_i \notin \text{span}(\{\veca_j\}_{j\neq i})$ as the columns of $\mA$ are linearly independent. Furthermore, the null space of $\mA_{-i}^\top$ is the orthogonal complement of the span of the columns of $\mA_{-i}$, i.e., $\mathcal{N}(\mA_{-i}^\top) = \text{span}(\{\veca_j\}_{j\neq i})^\perp$. 

    Now, \emph{let us assume, for the sake of contradiction that} for each $\vt \in \R^p$ such that $\mA_{-i}^\top \vt = \bm{0}$, we have $\veca_i^\top \vt = 0$. This would mean that 
    $$\mathcal{N}(\mA_{-i}^\top) \subset \veca_i^\perp.$$ 
    Taking orthogonal complement on both sides, we get 
    $$(\veca_i^\perp)^\perp \subset \mathcal{N}(\mA_{-i}^\top)^\perp.$$ 
    Note that, $(\veca_i^\perp)^\perp = \spn(\veca_i)$, and also that $\mathcal{N}(\mA_{-i}^\top)^\perp = \spn(\{\veca_j\}_{j\neq i})$. That is,
    $\spn(\veca_i) \subset \spn(\{\veca_j\}_{j\neq i}).$
    This is a contradiction. Thus, there exists a vector $\vt \in \R^p$ such that $\veca_i^\top \vt \neq 0$ and $\mA_{-i}^\top \vt = \bm{0}$.  
\end{proof}

\subsection{Proof of \texorpdfstring{\Cref{theorem:full-rank-possible}}{Theorem 4}}
\label{app:theorem-full-rank-possible-proof}

Before we prove the theorem above, we state a technical lemma from functional analysis which is utilized in the proof of the theorem. 

\begin{lemma}\label{app-lemma:non-trivial-polynomials}
Let $P: \R^n \to \R$ be a non-trivial polynomial, then the zero set of $P$ has zero Lebesgue measure.     
\end{lemma}

See~\cite{folland1999real} for more details on \cref{app-lemma:non-trivial-polynomials}. We are now ready to prove \cref{theorem:full-rank-possible}

\begin{proof}[\Cref{theorem:full-rank-possible}]
    We divide the proof into two parts. In part 1, we show the existence of a measurement matrix $\mA_0$ that is not a part of $\bar{\mathcal{A}}$. Then, in part 2, using the result from part 1 we then conclude that the set $\bar{\mathcal{A}}$ has zero Lebesgue measure. 
    
    \vspace{0.3cm}
    \noindent
    \emph{Part 1: Existence of a measurement matrix $\mA_0$ such that $\mT_2$ is full rank}

    \vspace{0.3cm}
    \noindent
    For $p \geq d$, let us define $\mA_0$ as follows: 
    $$
    \mA_0 = \begin{bmatrix}
    \mI_d\\
    \mathbf{0}
    \end{bmatrix}, \quad \text{i.e., }\veca_{0,i} = \ve_i \text{ for } i = 1, \ldots, d. 
    $$
    For $i = 1, \ldots, d$, let $\vt^{(i)} = \ve_i$, and for $i = d+1, \ldots, p$, let $\vt^{(i)} = \ve_1 + \ve_i$. It is easy to check that $\{\vt^{(1)}, \ldots, \vt^{(p)}\} \subseteq \mathcal{T}(\mA_0)$. Thus, $\mT_2$ takes the following form: 
    $$
    \mT_2 = \begin{bmatrix}
    \mI_d & \mathbf{0}\\
    \mE_{1, p-d} & \mI_{p-d}\
    \end{bmatrix}
    $$
    where $\mE_{1, p-d} \in \R^{p-d \times d}$ denotes a matrix with ones in the first column and zeros everywhere else. Clearly, $\rank(\mT_2) = p$, i.e., $\mT_2$ is full rank. Thus, we have shown the existence of a non-trivial measurement matrix $\mA_0 \notin \bar{\mathcal{A}}$.  

    \vspace{1cm}
    \noindent
    \emph{Part 2: $\bar{\mathcal{A}}$ has zero Lebesgue measure}

    \vspace{0.3cm}
    \noindent
    Since $\rank(\mA) = d$, we know that $\rank(\mA_{-i}) = d-1$, and thus, $\mA_{-i}^\top \in \R^{(d-1) \times p}$ has rank $d-1$. Then, there exists a subset of rows $J_i \subset \{1, \ldots, p\}$, with $|J_i| = d-1$ such that the square matrix
    $$\mM_i(\mA) \triangleq (\mA_{-i})_{J_i, \ast} \in \R^{(d-1) \times (d-1)}$$
    is invertible. 

    Let $\vt$ be such that $\mA_{-i}^\top \vt = 0$ for some $i \in [d]$. Then, 
    $$\mM_i(\mA)^\top\vt_{J_i} + \mR_i(\mA)^\top\vt_{[p] \setminus J_i} = 0,$$
    where $\mR_i(\mA)$ denotes the submatrix of $\mA$ formed by rows not included in $J_i$. Since $\mM_i(\mA)$ is invertible, we have
    $$\vt_{J_i} = -\Big(\mM_i(\mA)^\top\Big)^{-1}\mR_i(\mA)^\top\vt_{[p] \setminus J_i}.$$
    Thus, every admissible $\vt$ has to have the following form: 
    $$
    \vt(\mA, \vecu) = \begin{bmatrix}
    -\Big(\mM_i(\mA)^\top\Big)^{-1}\mR_i(\mA)^\top\vecu\\
    \vecu
    \end{bmatrix}, \quad \vecu \in \R^{p-d}.
    $$
    Moreover, 
    $$\mM_i(\mA)^{-1} = \frac{\text{adj}(\mM_i(\mA))}{\det(\mM_i(\mA))}$$
    Thus, the each coordinate of $\vt(\mA, \vecu)$ are: linear in $\vecu$, divided $\det(\mM_i(\mA))$, and multiplied by polynomial functions of entries of $\mA$. Upon taking Hadamard product with itself, each entry of $\vt^\odot$ is a polynomial function of $\vecu$ and the entries of $\mA$ divided by the determinant of the minor matrices.

    Suppose we choose $p$ such vectors $\vt^{(1)}, \ldots, \vt^{(p)}$ (each possibly corresponding to different column of $\mA$). The determinant of the resulting $\mT_2$, $\det(\mT_2)$ is also polynomial in $\vecu^{(\ell)}$, for $\ell \in [p]$; and polynomial in entries of $\mA$  along with a division of the determinant of the minor matrices. That is, 
    $$\det(\mT_2) = \frac{\text{Polynomial in } \mA, \vecu^{(1)}, \ldots, \vecu^{(p)}}{\prod_{\ell=1}^p \det(\mM_\ell(\mA))^{k_\ell}}$$

    Let us define $$D(\mA) \triangleq \prod_{\ell=1}^p \det(\mM_\ell(\mA))^{k_\ell}$$ and $$P(\mA, \vecu^{(1)}, \ldots, \vecu^{(p)}) \triangleq D(\mA) \cdot \det(\mT_2). $$

    Note that, since the minor matrices are invertible 
    $$P(\mA, \vecu^{(1)}, \ldots, \vecu^{(p)}) = 0 \iff \det(\mT_2) = 0. $$

    In \emph{Part 1}, we showed the existence of an $\mA_0$ and $\vecu_0^{(1)}, \ldots, \vecu_0^{(p)}$ for which the function $P(\mA_0, \vecu_0^{(1)}, \ldots, \vecu_0^{(p)}) \neq 0$. Thus the polynomial $P$ is non-trivial. Hence, from \cref{app-lemma:non-trivial-polynomials}, the zero set of $P$ has zero Lebesgue measure. Thus, $\bar{\mathcal{A}}$---which is a subset of the zero set of $P$---has zero Lebesgue measure. 
\end{proof}

\subsection{Proof of \texorpdfstring{\Cref{theorem:consistency}}{Theorem 5}}

\label{app:theorem-consistency-proof}

In this subsection we provide the proof of consistency of RECLAIM under exact maximization. We start by reviewing the relevant definitions and prior results required to prove \cref{theorem:consistency}. 

\subsubsection{Preliminaries} 

Consider a directed graph $\gr = (\sx, \se)$. A \emph{path} $\pi$ between nodes $X_i$ and $X_k$ is a sequence of nodes $(X_{i_0}, X_{i_1}, \ldots, X_{i_n})$, with $X_{i_0} = X_i$, $X_{i_n} = X_k$, and every two consecutive nodes in the sequence are connected by an edge, i.e., either $X_{i_j} \to X_{i_{j+1}} \in \se$ or $X_{i_j} \gets X_{i_{j+1}} \in \se$ for all $j = 0, \ldots, n-1$, with $X$. A path is \emph{directed} if all the edges from $X_i$ to $X_k$ are oriented the same way. A cycle through node $X_i$ consists of a directed path from $X_i$ to a node $X_j$ and the directed edge $X_j \to X_i$. For a node $X_i$, the set of \emph{ancestors} is defined as $\text{an}_\gr(X_i) := \{X_j \in X \mid \text{a directed path exists between } X_j \text{ and } X_i\}$. Similarly, the \emph{descendant} of a node is defined as $\text{de}_\gr(X_i) := \{X_j \in X \mid \text{a directed path exists between } X_i \text{ and } X_j\}$. The \emph{strongly connected component} of a node $X_i$ is given by the intersection of the ancestors and the descendants of $X_i$, i.e., $\text{sc}_\gr(X_i) = \text{an}_\gr(X_i) \cap \text{de}_\gr(X_i)$. We can apply these definitions to subsets $\sx_U$ by taking the union over all the elements in the subset, i.e., $\text{de}_\gr(\sx_U) = \cup_{i \in U} \text{de}_\gr(X_i)$. Finally, a node $X_i$ is called a \emph{collider} in a path $\pi$ if it satisfies the following two conditions: (i) it is a non-endpoint node, and (ii) the subpath $(X_k, X_i, X_j)$ is of the form $X_k \to X_i \gets X_j$. 

In a cyclic graph, the notion of $\sigma$-separation was introduced by~\cite{forre2017markov} to relate structural properties in the graph to independencies observed in the generated distribution. 

\begin{definition}[$\sigma$-separation]
    Let $\gr = (\sx, \se)$ be a directed graph and let $\sx_C \subseteq \sx$ be a subset of nodes. A path $\pi = (X_{i_0}, X_{i_1}, \ldots, X_{i_n})$ is said to be $\sigma$-blocked given $\sx_C$ if 
     \begin{enumerate}
         \item the first node of $\pi$, $X_{i_0} \in \sx_C$ or its last node $X_{i_n} \in \sx_C$, or 
         \item $\pi$ contains a collider $X_j \notin \sx_C$,
         \item $\pi$ contains a non-collider $X_j \in \sx_C$ that points towards a neighbor that is not in the same strongly connected component as $X_j$ in $\gr$, i.e., $X_k \gets X_j \in \pi$ and $X_k \notin \text{sc}_\gr(X_j)$, or $X_j \to X_\ell \in \pi$ and $X_\ell \notin \text{sc}_\gr(X_j)$. 
    \end{enumerate}
     The path $\pi$ is said to be $\sigma$-open given $\sx_C$ if it is not $\sigma$-blocked. Two subsets of nodes $\sx_A, \sx_B \subseteq \sx$ is said to be $\sigma$-separated given $\sx_C$ if all the paths between $X_a$ and $X_b$, where $a \in A$ and $b \in B$, are $\sigma$-blocked given $\sx_C$, and is denoted by
     $$\sx_A \mathop{\perp}_{\gr}^{\sigma} \sx_B \mid \sx_C.$$
\end{definition}

When the graph is cyclic, $\sigma$-separation defined above reduces to the standard $d$-separation. We node define the property that connects $\sigma$-separations with distributional independencies. 

\begin{definition}[General directed global Markov Property~\citep{forre2017markov}]
    Let $\gr = (\sx, \se)$ be a directed graph and $p$ denote the probability density of the observations $\sx$. The probability density $p$ satisfies the \emph{general directed global Markov property} if for $\sx_A, \sx_B, \sx_C \subseteq \sx$
    $$\sx_A \mperp_\gr^\sigma \sx_B \mid \sx_C \implies \rvx_A \mperp_{p} \rvx_B \mid \rvx_C,$$
    where $\rvx_A \mperp_{p} \rvx_B \mid \rvx_C,$ denotes conditionally independence of $\rvx_A$ and $\rvx_B$ given $\rvx_C$ with respect to $p$. 
\end{definition}

\paragraph{Joint causal modeling of interventions.} We adopt the \emph{joint causal inference} (JCI) framework proposed by~\cite{mooij2020joint} to unify multiple interventional settings into a single representative system. This is done by augmenting the system with context variables $\sce_\si = (\rvc_1, \ldots, \rvc_K)$, where $\rvc_k$ corresponds to the $k$-th interventional setting $I_k$, we call this the \emph{meta system}. We consider the system to be under the $k$-th interventional setting when $\rvc_j = \emptyset$ for $j \neq k$ and $\rvc_k = \bm{\xi}_{I_k}$ where $\bm{\xi}_{I_k} \in \R^{|I_k|}$. Additionally, we construct an augmented graph $\gr^\si$ consisting of both the latent system variables $\sx$ and the context variables $\sce_\si$. The children of each context variable $\rvc_k$ are the interventional targets in $I_k$, i.e., $\text{ch}_{\gr^\si}(\rvc_k) = \sx_{I_k}$. Note that there are no edges going from variables in $\sx$ to the context variables $\sce_\si$, \seeref{app-fig:aug-graph}. Finally, given a family of interventional targets $\si = \{I_k\}_{k=1}^K$, and the corresponding context variables $\sce_\si$, the structural equations governing the meta system is given by   
\begin{equation*}
    \tilde{f}_i(\pa_{\gr^\si}(X_i), Z_i) = \begin{cases}
        (\rvc_k)_i & \text{if }, \exists k \in [K] \text{s.t. } \rvc_k \neq\emptyset, X_i \in \sx_{I_k},\\
        f_i(\pa_\gr(X_i)) + Z_i, & \text{otherwise}.\\
    \end{cases}
\end{equation*}
Note that $\pa_{\gr^\si}(X_i)$ includes both latent system variables and the context variables. The meta-SCM above defines a probability distribution over the joint meta-system variables: 
\begin{equation}\label{app-eq:meta-prob-density}
    p_{\gr^\si}(\rvx, \sce_\si) = p_{\gr^\si}(\sce_\si)p_{\gr^\si}(\rvx\mid\sce_\si),
\end{equation}
where $p_{\gr^\si}(\sce_\si)$ is called the \emph{context distribution} and as noted by~\cite{mooij2020joint}, the behavior of the system is unaffected by the context distribution. Furthermore, when $\rvc_k = \emptyset$ for all $k \in [K]$, $p_{\gr^\si}(\rvx\mid\sce_\si)$ becomes the observational data, and
$$
p_{\gr^\si}(\rvx \mid \rvc_k = \bm{\xi}_{I_k}, \rvc_{-k} = \emptyset) = p_{\tdo(I_k)(\gr)}(\rvx).
$$
Recall, for the interventional setting $I_k$, probability density governing the latents $\rvx$ is given by \cref{eq:prob-density-interventions} which we repeat here for convenience
\begin{equation*}
    p_{\tdo(I)(\gr)}(\rvx) = p_C(\rvx_I)p_Z\big(\rvz_{[d]\setminus I}\big)\big|J_{(\id - \mU f)}(\rvz)\big|.
\end{equation*}

\begin{figure}[t]
\centering 
\input{app-figures/augmented-graph}
\caption{Illustration of the augmented graph $\gr^\si$ corresponding the set of interventional targets $\si = \{\emptyset, \{1\}, \{3\}\}$. (b) and (c) represent the mutilated graph obtained after interventions on $X_1$ and $X_3$ respectively. The augmented graph is the union of $\gr$, $\tdo(\{X_1\})(\gr)$, and $\tdo(\{X_3\})(\gr)$ along with the context variables $C_1$ and $C_2$. } 
\label{app-fig:aug-graph}
\end{figure}

\begin{definition}
    Let $\gr = (\sx, \se)$ be a directed graph, and $\si = \{I_k\}_{k=1}^K$ be a family of interventional experiments. Let $\sm_\si(\gr)$ denote the set of positive densities $p_{\gr^\si} : \R^{2d} \to \R$ such that $p_{\gr^\si}$ is given by \cref{app-eq:meta-prob-density} for all $f:\R^{d} \to \R^d$, with $f_i(\rvx) = f_i({\pa_\gr}(X_i))$, such that the resulting forward map $(\id - f)$ is a diffeomorphism, for all $(\sigma_{Z, 1}^2, \ldots, \sigma_{Z,d}^2)$ such that $\rvz \sim \mathcal{N}\big(0, \text{Diag}(\sigma_{Z,1}^2, \ldots, \sigma_{Z,K}^2)\big)$.
\end{definition}

$\sm_\si(\gr)$ denotes the set of interventional density generated by $\gr^\si$. We now show that these densities satisfy the general directed global Markov property.

\begin{prop}\label{app-prop:general-markov-property}
    Let $\gr = (\sx, \se)$ be a directed graph, and $\si = \{I_k\}_{k=1}^K$ be a family of interventional experiments, let $p \in \sm_\si(\gr)$, then $p$ satisfies the general directed global Markov property relative to $\gr^\si$.
\end{prop}

\begin{proof}
    For a directed graph $\gr$ and a choice of $f : \R^{d} \to \R^d$ such that the forward map $(\id - f)$ is a diffeomorphism, the structural equations are uniquely solvable with respect to each strongly connected component of $\gr$. Moreover, since the addition of context variable doesn't introduce any cycles, from~\cite[Theorem A.21]{bongers2021foundations}, the distribution $p_{\gr^\si}$ is unique and it satisfies the general directed global Markov property. 
\end{proof}

Given a family of interventional experiments, we now define a notion of an equivalence class of directed (cyclic) graphs based on the set of distributions induced by them. 

\begin{definition}[$\si$-Markov Equivalence Class]
    Two directed graphs $\gr$ and $\gr^\prime$ are $\si$-Markov equivalent if and only if $\sm_\si(\gr) = \sm_\si(\gr^\prime)$, denoted as $\gr \equiv_\si \gr^\prime$. The set of all directed graphs that are $\si$-Markov equivalent to $\gr$ is the $\si$-Markov equivalence class of $\gr$, denoted as $\si$-MEC$(\gr)$. 
\end{definition}

\subsubsection{Proof of \texorpdfstring{\Cref{theorem:consistency}}{Theorem 5}} 

We now prove the main theoretical contribution of this work. Recall the score function defined in \cref{sec:reclaim-score}
\begin{equation*}
    \score_\si(\gr) \triangleq \sup_{\vtheta, \vphi} \sum_{k=1}^K \expect_{\rvy \sim p^{(k)}} 
    \log p(\rvy \mid \vtheta, \vphi, I_k) - \lambda|\gr|,
\end{equation*}
where  $p^{(k)}$ is the true data-generating distribution for \( \si = \{I_k\}_{k=1}^K \), and $(\vtheta, \vphi)$ represents the model parameters (latent SCM and measurement process). In the context of the meta system, the score function above is equivalent to the following score: 
\[
\score_\si(\gr) \triangleq \sup_{\vtheta, \vphi} \expect_{(\rvy, \rvc) \sim p_\si^\ast} \log p_{\gr^\si}(\rvy, \rvc \mid \vtheta, \vphi) - \lambda |\gr|,
\]
where $p_\si^\ast$ denotes the joint ground-truth distribution for the observed and the context variables, and $p_{\gr^\si}(\rvy, \rvc \mid \vtheta)$ is given by 
\begin{equation}\label{app-eq:obs-to-latent-map}
p_{\gr^\si}(\rvy, \rvc \mid \vtheta, \vphi) = \int_{\rvx} p(\rvy \mid \rvx, \vphi) p_{\gr^\si}(\rvx, \rvc \mid \vtheta)\,d\rvx.    
\end{equation}
Note that $p(\rvy \mid \rvx, \vphi)$ is defined by the measurement process $g(\rvx, \rve)$. 

We define \( \spe_\si(\gr) \) as the set of all distributions \( p_{\gr^\si}(\rvx, \rvc  \mid \vtheta)\) that can be expressed by the model specified by \cref{eq:sem-combined,eq:prob-density-interventions} in the main paper, and \cref{app-eq:meta-prob-density}. That is,
$\spe_\si(\gr) := \{p \mid \exists\,\vtheta \text{ s.t } p = p_{\gr^\si}(\cdot \mid \vtheta)\}$. Thus, it is clear that $\spe_\si(\gr) \subseteq \sm_\si(\gr)$. Similarly, we define the of observed distributions expressable by $\gr$, denoted as $\spe_{Y, \si}(\gr) = \{p \mid \exists (\vtheta, \vphi) \text{ s.t. } p = p_{\gr^\si}(\cdot \mid \vtheta, \vphi)\}$. In the following proposition we show that $\spe_{Y, \si}(\gr)$ is uniquely determined by a $p \in \spe_\si(\gr)$ when $\si$ satisfies \cref{cond:channel-indentifiability-interventions}.

\begin{prop}\label{app-prop:map-injectivity}
    Let $\si = \{I_k\}_{k=1}^K$ be a family of interventional experiments satisfying \cref{cond:channel-indentifiability-interventions}. Then for a fixed set of measurement parameters $\vphi$, under both Gaussian additive noise (GAN) measurement process and linear measurement system, the map $T: \spe_\si(\gr) \to \spe_{Y, \si}(\gr)$ given by \cref{app-eq:obs-to-latent-map} is injective. 
\end{prop}

\begin{proof}
    Under \cref{cond:channel-indentifiability-interventions}, the measurement noise variance is fully identifiable (\seeref{sec:measurement-system-estimate} for more details). For sake of simplicity, let us assume that the noise variances are equal (the conclusion even otherwise) and set to $\sigma^2$. Taking the characteristic functions of $Tp = Tp^\prime$ and dividing by the non-vanishing Gaussian factor $e^{-\sigma^2\norm{\bm{\xi}}^2/2}$ yields $\expect_p [e^{-i\bm{\xi}^\top h(\rvx)}] = \expect_{p^\prime} [e^{-i\bm{\xi}^\top h(\rvx)}]$ for all $\bm{\xi}$. Here, $f(\rvx) = \rvx$ for GAN system and $f(\rvx) = \mA\rvx$ for linear measurement system. Thus, from the uniqueness of the characteristic function~\citep{billingsley1995probability}, $f_\#p = f_\#p^\prime$. Since $f$ is injective, $p = p^\prime$. 
\end{proof}

\Cref{theorem:consistency} relies on the following set of assumptions. The first one ensures that the model is capable of representing the ground truth distribution. 

\begin{assume}[Sufficient Capacity] \label{app-assume:sufficient-capacity}
    The joint ground truth distribution $p_\si^\ast$ is such that $p_\si^\ast \in \spe_\si(\gr^\ast)$, where $\gr^\ast$ is the ground truth latent graph. 
\end{assume}

In other words, there exists a $\vtheta$ such that $p_\si^\ast = p_{\gr^\si}(\cdot \mid \vtheta)$. The second assumption generalizes the notion of faithfulness assumption to the interventional setting. 

\begin{assume}[$\si$-$\sigma$-faithfulness]\label{app-assume:faithfulness}
For any subset of nodes $A, B, D \subseteq \sx \cup \sce_\si$, and $I_k \in \si$
$$A \mathop{\not\perp}_{\gr^\si}^\sigma B \mid D \implies \bm{A} \mathop{\not\perp}_{p_{\gr^\si}} \bm{B} \mid \bm{C}. $$
\end{assume}

The above assumption implies that any conditional independency observed in the data must imply a $\sigma$-separation in the corresponding interventional ground truth graph. 

\begin{assume}[Strict positivity]\label{app-assume:positivity}
    For all $(\rvx, \rvc)$ and $p_{\gr^\si} \in \sm_\si(\gr)$, $p_{\gr^\si}(\rvx, \rvc) > 0$. 
\end{assume}

\begin{assume}[Finite differential entropy]\label{app-assume:finite-entropy}
    For a family of interventions $\{X_{\si_m}\}_{m=0}^M$,
    $$ \abs{ \expect_{p_\si^\ast}\log p_\si^\ast(\rvy, \rvc) } < \infty.$$
\end{assume}

The last two assumptions ensure that the scenario where $\score(\gr^\ast)$ and $\score(\gr)$ are both infinity is avoided. This is formalized in the lemma below taken from~\cite{brouillard2020differentiable}. 

\begin{lemma}[Finiteness of the score function \citep{brouillard2020differentiable}]
    Under the \cref{app-assume:sufficient-capacity,app-assume:finite-entropy}, the score function is finite, that is, $|\score_\si(\gr)| < \infty$. 
\end{lemma}

We finally make the assumption that the parameter space of $\vtheta$ and $\vphi$ are compact. 

\begin{assume}[Parameter compactness]\label{app-assume:parameter-compactness}
    The parameters of the measurement process $\vphi$ belong to a compact metric space $\Phi$.  
\end{assume}

For the both Gaussian additive noise (GAN) and linear measurement system, the parameters correspond to the variance of the Gaussian distribution, $\vphi = (\sigma_1^2, \ldots, \sigma_p^2)$. For the case of GAN system, $p = d$. The implication of the above assumption is that $\sigma_j^2 \leq \sigma_{\max}^2$, i.e., it is bounded above. Additionally, note that since we restrict the causal mechanism to \emph{contractive}, the parameters of latent SCM also belong to a compact space. 

From the results of~\cite{brouillard2020differentiable}, we can now express the difference in score function between $\gr^\ast$ and $\gr$ as the minimization of KL diverengence plus the difference in the regularization terms. 

\begin{lemma}[Rewritting the score function \citep{brouillard2020differentiable}]\label{app-lemma:scores}
    Under assumptions \ref{app-assume:sufficient-capacity} and \ref{app-assume:finite-entropy}, we have 
    $$\score(\gr^\ast) - \score(\gr) = \inf_{\vtheta, \vphi} D_{KL}(p_{\si}^\ast\| p_{\gr^\si}(\cdot \mid \vtheta, \vphi)) + \lambda (|\gr| - |\gr^\ast|).$$
\end{lemma}

Furthermore, \cite{sethuraman2025differentiable} showed that the KL divergence appearing the in lemma above is strictly positive when the latent variables are directly observed. 

\begin{lemma}[Lemma A.18 \citep{sethuraman2025differentiable}]\label{app-lemma:strictly-pos}
    Let $\gr = (\sx, \se)$ be a directed graph, for a set of interventional targets $\si = \{I_k\}_{k=1}^K$, and $p^\ast \notin \sm_\si(\gr)$, then
    $$\inf_{p\in \sm_\si(\gr)} D(p^\ast\|p) > 0.$$
\end{lemma}

We now extend this result to the case of indirect measurements. 

\begin{lemma}\label{app-lemma:strictly-pos-obs}
    Let $\gr = (\sx, \se)$ be a directed graph, for a set of interventional targets $\si = \{I_k\}_{k=1}^K$ satisfying \cref{cond:channel-indentifiability-interventions}, and $p^\ast_Y \notin \sm_{Y,\si}(\gr)$, then
    $$\inf_{p\in \sm_{Y, \si}(\gr_m)} D(p^\ast_Y\|p_Y) > 0.$$
\end{lemma}

\begin{proof}
Since $\si$ satisfies \cref{cond:channel-indentifiability-interventions}, the parameters of the measurement process is fully identified. Moreover, from \cref{app-prop:map-injectivity}, the map $T: \spe_\si(\gr) \to \spe_{Y, \si}(\gr)$. Thus, $T^{-1}p_Y^\ast \notin \spe_\si(\gr)$. Thus, from \cref{app-lemma:strictly-pos}, no sequence $\{p^{(k)}\}_{k=1}^\infty \subset \sm_si(\gr)$ exists such that the limit $\lim_{k\to\infty} p^{(k)} = T^{-1}p_Y^\ast$. Therefore, there exists no sequence $\{p_Y^{(k)}\}_{k=1}^\infty \subset \sm_{Y,si}(\gr)$ such that $\lim_{k\to\infty} p_Y^{(k)} = p_Y^\ast$. Thus,
$$\inf_{p\in \sm_{Y, \si}(\gr_m)} D(p^\ast_Y\|p_Y) > 0. $$
This proves the lemma.
\end{proof}

We are now ready to prove \cref{theorem:consistency}. Recall,

\begin{customthm}{\ref{theorem:consistency}.}
    Let $\si = \{I_k\}_{k=1}^K$ be a family of interventional targets satifying \cref{cond:channel-indentifiability-interventions}, let $\gr^\ast$ denote the ground truth directed graph, $p^{(k)}$ denote the data generating distribution for $I_k \in \si$, and $\hat{\gr} := \arg\max_{\gr} \score(\gr)$. Then, under \cref{app-assume:sufficient-capacity,app-assume:faithfulness,app-assume:positivity,app-assume:finite-entropy,app-assume:parameter-compactness}, and for a suitably chosen $\lambda > 0$, we have that $\hat{\gr} \equiv_\si \gr^\ast$. That is, $\hat{\gr}$ is $\si$-Markov equivalent to $\gr^\ast$.
\end{customthm}

\begin{proof}
The proof is a direct extension of Theorem 2 in \cite{sethuraman2025differentiable}, with \cref{app-lemma:strictly-pos-obs} substituting \cref{app-lemma:strictly-pos}. Which we present here for self-containment. 

It is sufficient to show that for $\gr \notin \si\text{-MEC}(\gr^\ast)$, the score function of $\gr$ is strictly lower than the score function of $\gr^\ast$, i.e., $\score(\gr^\ast) > \score(\gr)$. Since \( \gr \notin \si\text{-MEC}(\gr^\ast) \) and \( p_\si^\ast\in \sm_\si(\gr^\ast) \) (by \cref{app-assume:sufficient-capacity}), there must exist subsets of nodes \( A, B, D \subseteq \sx \cup \sce_\si \) such that either:
\begin{equation}\label{eq:condition-1}
A \mperp_{\gr}^\sigma B \mid D \quad \text{and} \quad A \mathop{\not\perp}_{\gr^\ast}^\sigma B \mid D, \tag{C1}
\end{equation}
or
\begin{equation}\label{eq:condition-2}
A \mathop{\not\perp}_{\gr}^\sigma B \mid D \quad \text{and} \quad A \mperp_{\gr^\ast}^\sigma B \mid D, \tag{C2}   
\end{equation}
If no such subsets exist, then \( \gr \) and \( \gr^\ast \) impose the same  $\sigma$ -separation constraints and thus induce the same set of distributions. This would imply that \( \gr \in \si\text{-MEC}(\gr^\ast) \), contradicting our assumption. Since $p_\si^\ast \in \sm_\si(\gr^\ast)$, in the case of \eqref{eq:condition-1}, it must be true that $\bm{A} \not\perp_{p_\si^\ast} \bm{B} \mid \bm{D}$ (\cref{app-assume:faithfulness}). Therefore $p_\si^\ast$ doesn't satisfy the general directed Markov property with respect to $\gr^\si$ and hence $p_\si^\ast \notin \sm_\si(\gr)$. For \eqref{eq:condition-2}, if $p_\si^\ast \in \sm_\si(\gr)$, then from \cref{app-assume:faithfulness}, it must be true that $\bm{A} \not\perp_{p_\si^\ast} \bm{B} \mid \bm{C}$. However, $p_\si^\ast \in \sm_\si(\gr^\ast)$, and \cref{app-prop:general-markov-property} implies that $\bm{A} \perp_{p_\si^\ast} \bm{B} \mid \bm{C}$, resulting in a contradiction. Therefore, $p_\si^\ast \notin \sm_\si(\gr)$. Morevover, from \cref{app-prop:map-injectivity} we can conclude that $p_{Y, \si}^\ast \notin \sm_{Y, \si}(\gr)$.  

For convenience, let $$\eta(\gr) := \inf_{\vtheta} D_{KL}(p_{Y,\si}^\ast\|p_{Y, \gr^\si}(\cdot \mid \vtheta, \vphi^\ast)).$$
Note that
$$\eta(\gr) = \inf_{\vtheta} D_{KL}(p_{Y,\si}^\ast\|p_{Y, \gr^\si}(\cdot \mid \vtheta, \vphi^\ast)) \geq \inf_{p \in \sm_{Y,\si}(\gr)} D_{KL}(p_Y^{(k)}\|p_Y) > 0,$$
where we use \cref{app-lemma:strictly-pos-obs} for the final inequality. Thus, from Lemma~\ref{app-lemma:scores}
\begin{equation*}
    \score(\gr^\ast) - \score(\gr) = \eta(\gr) + \lambda(|\gr| - |\gr^\ast|).
\end{equation*}
Following \cite{brouillard2020differentiable}, we now show that by choosing $\lambda$ sufficiently small, the above equation is stictly positive. Note that if $|\gr| \geq |\gr^\ast|$ then $\score(\gr^\ast) - \score(\gr) > 0$. Let $\mathbb{G}^+ := \{\gr \mid |\gr| < |\gr^\ast|\}$. Choosing $\lambda$ such that $0 < \lambda < \min_{\gr \in \mathbb{G}^+} \frac{\eta(\gr)}{|\gr^\ast| - |\gr|}$ we see that: 
\begin{align*}
    &\lambda < \min_{\gr \in \mathbb{G}^+} \frac{\eta(\gr)}{|\gr^\ast| - |\gr|}\\
    \iff &\lambda < \frac{\eta(\gr)}{|\gr^\ast| - |\gr|} \quad \forall \gr \in \mathbb{G}^+\\
    \iff &\lambda (|\gr^\ast| - |\gr|) < \eta(\gr) \quad \forall \gr \in \mathbb{G}^+\\
    \iff & 0 < \eta(\gr) + \lambda(|\gr| - |\gr^\ast|) = \score(\gr^\ast) - \score(\gr) \quad \forall \gr \in \mathbb{G}^+.
\end{align*}
Thus, every graph outside of the general directed Markov equivalence class of $(\gr^\ast)^\si$ has a strictly lower score. 
\end{proof}

% Section containing additional implementation details

\section{Implementation Details}
\label{app:implementation-details}

In this section we provide further technical details on the implementation of RECLAIM and the baselines. 

\subsection{Projection Vector Sampling for Measurement Noise Estimation}
\label{app:projection-sampling}

The overall projection vector sampling algorithm for noise variance estimation is summarized in \cref{app-alg:projection-sampling}. We start with an empty $\mT_2$ matrix and iterating through each node in the latent graph. For each $i \in [d]$, let $\mM_i$ be the measurement matrix $\mA$ excluding the $i$-th column. We then compute its singular value decomposition (SVD) and extract the columns of $\mV$ matrix corresponding to zero singular values, denoted as $\mB_i$. These columns represent the basis vectors of the null space of $\mM_i$. A random vector $\vecu$ is then generated to obtain the projection matrix $\vt = \mB_i\vecu$. The vector $\vt$ is appended to $\mT_2$ if it provided sufficient signal and is sufficiently diverse from the existing projection vectors already in $\mT_2$. The process concludes once we sample the required number of rows for $\mT_2$. \Cref{theorem:full-rank-possible} guarantees that the above procedure would conclude and the results matrix $\mT_2$ would be full (column) rank. 

\begin{algorithm}[t]
\caption{Sampling Projection Vectors for Noise Estimation}
\label{app-alg:projection-sampling}
\begin{algorithmic}[1]
\Require Measurement matrix $\mA \in \R^{p \times d}$, intervention family $\si$ 
satisfying \cref{cond:channel-indentifiability-interventions}, thresholds 
$\epsilon_\text{sig} > 0$, $\delta > 0$, target number of vectors $m$
\Ensure Projection matrix $\mT_2 \in \R^{m \times p}$
\State Initialize $\mT_2 \leftarrow [\,]$
\For{$i = 1, \ldots, d$}
    \State Compute $\mM_i \leftarrow \mA_{-i}^\top \in \R^{(d-1) \times p}$
    \State Compute SVD: $\mM_i = \mU \mSigma \mV^\top$
    \State Extract basis $\mB_i \in \R^{p \times r}$ from columns of $\mV$ corresponding 
    to zero singular values, where $r = p - d + 1$
    \While{fewer than $\lfloor m/d \rfloor$ vectors collected for node $i$}
        \State Sample $\vecu \sim \mathcal{N}(\bm{0}, \mI_r)$
        \State Set $\vt \leftarrow \mB_i \vecu$
        \If{$|\veca_i^\top \vt| < \epsilon_\text{sig}$} \Comment{weak signal}
            \State \textbf{reject} and \textbf{continue}
        \EndIf
        \State Normalize: $\vt \leftarrow \vt / \|\vt\|$
        \If{$\exists\, (\vt^\prime)^{\odot} \in \mT_2$ s.t. $\cos\big(\vt^{\odot}, 
        (\vt^\prime)^{\odot}\big) > 1 - \delta$} \Comment{insufficient diversity}
            \State \textbf{reject} and \textbf{continue}
        \EndIf
        \State Append $(\vt^\odot)^\top$ to $\mT_2$
    \EndWhile
\EndFor
\State \Return $\mT_2$
\end{algorithmic}
\end{algorithm}

\subsection{Log-determinant of the Jacobian Computation}
\label{app:log-det-jacobian}

Computing the log-determinant of the Jacobian computation poses a significant challenge when evaluation the log-density of the latent variables. To overcome this issue, we exploit the power-series expansion of $\log(1 - x)$ to obtain the following: 
\begin{equation}
    \log \big|\det J_{(\id - \mU f)}(\rvx)\big| = 
    -\sum_{m=1}^\infty \frac{1}{m} \mathrm{Tr}\Big\{J^m_{\mU f}(\rvx)\Big\}.
    \label{app-eq:power-series}
\end{equation}
This brings the complexity of down to $\mathcal{O}(d^2)$. Further improvement can be made by using \emph{Hutchinson trace estimator}~\citep{hutchtraceestimator}
$$\mathrm{Tr}\Big\{J^m_{\mU f}(\rvx)\Big\} = \expect_{\mW}\Big[\mW^\top J^m_{\mU f}(\rvx)\mW\Big],$$
where $\mathbb{E}[\mW] = 0$ and $\mathbb{E}[\mW\mW^\top] = \mI$. The above estimator only depends on a vector-Jacobian product which can be efficiently computed using an auto-differentiation library (such as PyTorch), often reducing the complexity to $\mathcal{O}(d)$. In practice, the power series is truncated to a finite number of terms. This, however, introduces bias in the log-determinant of the Jacobian estimate. To improve on this, following~\cite{russianroulette}, the series cut-off $n$ is randomly sampled, $n \sim p_N$, where $p_N$ is a distribution over natural numbers $\mathbb{N}$. The individual terms in \cref{app-eq:power-series} are then reweighted by the inverse probability of ending there. Finally, we have the following unbiased estimator: 
\begin{equation}\label{app-eq:unbiased-log-det}
    \log \big|\det J_{(\id - \mU f)}(\rvx)\big| = 
    -\expect_{n, \mW} \Bigg[\sum_{m=1}^n \frac{\mW^\top J^m_{\mU f}(\rvx)\mW}{m\cdot P(N\geq n)} \Bigg].
\end{equation}

\subsection{RECLAIM and Baselines Code Details}

\paragraph{RECLAIM.} Our framework was built using the \texttt{Pytorch} library in Python and the code is provided as a part of the supplementary materials. 

We follow the setup of \cite{sethuraman2023nodags}, employing neural networks (NNs) with dependency masks parameterized by a Gumbel-softmax distribution. The log-determinant of the Jacobian is computed using a power series expansion combined with the Hutchinson trace estimator. To mitigate bias from truncating the power series expansion, the number of terms is sampled from a Poisson distribution, as detailed in \cref{sec:reclaim,app:log-det-jacobian}. The final objective is optimized using the Adam optimizer \citep{kingma2015adam}.

The learning rate in all our experiments was set to $10^{-2}$. The neural network models used in our experiments contained one multi-layer perceptron layer and \texttt{tanh} activation. The graph sparsity regularization constant $\lambda$ was set to $10^{-3}$ for all the experiments. The models were trained and evaluated on NVIDIA RTX6000 GPUs. 

\paragraph{Baselines. } For NODAGS-Flow, we used the code provided by authors \citep{sethuraman2023nodags} available at \url{https://github.com/Genentech/nodags-flows}. The default values were set for the hyperparameters. For DCDI, we used the codebase provided by the authors \citep{brouillard2020differentiable}, available at \url{https://github.com/slachapelle/dcdi}. The default hyperparameters were used while training and evaluating the model. For Anchored-CI, we implemented Algorithm 1 in~\citep{saeed2020anchored} using an implementation of PC algorithm available in \texttt{CausalDag} library in Python.

% Section containing additional experimental results
\section{Additional Experiments}
\label{app:additional-experiments}

% Colors for the baselines and RECLAIM
\def\colorRECLAIM{blue}
\def\colorNODAGS{green!80!black}
\def\colorDCDI{orange}
\def\colorAnchored{purple}

In all the experiments below, we fix $d=10$, $\sigma_{\min} = 0.3$, and $\sigma_{\max} = 0.6$. For linear measurement noise process, the number of measurements was fixed to $p=15$. 

\paragraph{Varying number of cycles.} We evaluate the sensitivity of RECLAIM to the number of cycles in the graph. The number of cycles was varied between 0 and 8 in steps of 2. The results are summarized in \cref{app-fig:varying-cycles}. The two cyclic graph methods (RECLAIM and NODAGS-Flow) remain stable across the entire range of varying cycles, whereas, the DAG methods (Anchored-CI and DCDI) exhibit a decreasing trend for both the noise processes. Overall RECLAIM outperforms all the baselines. 

\begin{figure}[ht]
    \centering
    \input{app-figures/varying-cycles.tex}
    \caption{Performance comparison with varying number of cycles in the latent variable graph.}
    \label{app-fig:varying-cycles}
\end{figure}

\paragraph{Varying degree of nonlinearity.} We evaluate the sensitivity of RECLAIM to the degree of nonlinearity of the latent data generation process. The latent variables are sampled from the following SCM: 
$$
\rvx = (1 - \beta) \mW^\top\rvx + \beta\tanh{\mW^\top\rvx} + \rvz,
$$
where $\beta$ controls the degree on nonlinearity. $\beta = 0$ corresponds to fully linear SCM and $\beta=1$ corresponds to fully nonlinear SCM. The results are summarized in \cref{app-fig:varying-nonlinearity}. As seen from the figure, RECLAIM exhibits robustness to nonlinearity in the data and achieves the best performance when compared to the baselines for all values of $\beta$. 

\begin{figure}[ht]
    \centering
    \input{app-figures/varying-beta.tex}
    \caption{Performance comparison with varying degree of nonlinearity in the latent variable SCM.}
    \label{app-fig:varying-nonlinearity}
\end{figure}

\paragraph{Varying latent graph sparsity.} We evaluate the sensitivity of RECLAIM to the sparsity of latent variable graph. The number of outgoing edge density of the latent variable graph was varied between 1 and 4. The results are summarized in \cref{app-fig:varying-graph-sparsity}. RECLAIM remains robust with respect to the recovery performance even as the latent graphs become more dense. NODAGS-Flow exhibits a decreasing trend in AUPRC score, while the DAG methods consistently score below the cyclic methods.  

\begin{figure}[ht]
    \centering
    \input{app-figures/varying-degree.tex}
    \caption{Performance comparison with varying latent graph sparsity.}
    \label{app-fig:varying-graph-sparsity}
\end{figure}

% \renewcommand{\arraystretch}{1.3}
% \setlength\tabcolsep{0.65em}
% \begin{table}[ht]
%     \centering 
%     \begin{tabular}{c|ccc|ccc}
%         \toprule
%         \multirow{2}{*}{\textbf{Sampler}} & \multicolumn{3}{c|}{\textbf{GAN}} & \multicolumn{3}{c}{\textbf{Linear Measurement}}\\ \cline{2-7}
%         & \textbf{AUPRC} & \textbf{SHD} & \textbf{Tr. Time} & \textbf{AUPRC} & \textbf{SHD} & \textbf{Tr. Time}\\   \hline\hline
%         SIR & 0.991 & 0.90 & 1.192 & 0.997 & 0.5 & 1.102\\
%         ULA & 0.993 & 1.30 & 3.389 & 0.954 & 3.10 & 3.267\\
%         Rejection & 0.977 & 2.25 & 11.256 & 0.997 & 0.5 & 8.27\\
%         \bottomrule
%     \end{tabular}    
% \end{table}
