# Supplementary material for: RECLAIM: Cyclic Causal Discovery Amid Measurement Noise
Source: arXiv:2603.20585 source file (2026-03-21)
Supplement: Supplementary file 2 [file additional-experiments.tex]

\section{Additional Experiments}
\label{app:additional-experiments}

% Colors for the baselines and RECLAIM
\def\colorRECLAIM{blue}
\def\colorNODAGS{green!80!black}
\def\colorDCDI{orange}
\def\colorAnchored{purple}

In all the experiments below, we fix $d=10$, $\sigma_{\min} = 0.3$, and $\sigma_{\max} = 0.6$. For linear measurement noise process, the number of measurements was fixed to $p=15$. 

\paragraph{Varying number of cycles.} We evaluate the sensitivity of RECLAIM to the number of cycles in the graph. The number of cycles was varied between 0 and 8 in steps of 2. The results are summarized in \cref{app-fig:varying-cycles}. The two cyclic graph methods (RECLAIM and NODAGS-Flow) remain stable across the entire range of varying cycles, whereas, the DAG methods (Anchored-CI and DCDI) exhibit a decreasing trend for both the noise processes. Overall RECLAIM outperforms all the baselines. 

\begin{figure}[ht]
    \centering
    \input{app-figures/varying-cycles.tex}
    \caption{Performance comparison with varying number of cycles in the latent variable graph.}
    \label{app-fig:varying-cycles}
\end{figure}

\paragraph{Varying degree of nonlinearity.} We evaluate the sensitivity of RECLAIM to the degree of nonlinearity of the latent data generation process. The latent variables are sampled from the following SCM: 
$$
\rvx = (1 - \beta) \mW^\top\rvx + \beta\tanh{\mW^\top\rvx} + \rvz,
$$
where $\beta$ controls the degree on nonlinearity. $\beta = 0$ corresponds to fully linear SCM and $\beta=1$ corresponds to fully nonlinear SCM. The results are summarized in \cref{app-fig:varying-nonlinearity}. As seen from the figure, RECLAIM exhibits robustness to nonlinearity in the data and achieves the best performance when compared to the baselines for all values of $\beta$. 

\begin{figure}[ht]
    \centering
    \input{app-figures/varying-beta.tex}
    \caption{Performance comparison with varying degree of nonlinearity in the latent variable SCM.}
    \label{app-fig:varying-nonlinearity}
\end{figure}

\paragraph{Varying latent graph sparsity.} We evaluate the sensitivity of RECLAIM to the sparsity of latent variable graph. The number of outgoing edge density of the latent variable graph was varied between 1 and 4. The results are summarized in \cref{app-fig:varying-graph-sparsity}. RECLAIM remains robust with respect to the recovery performance even as the latent graphs become more dense. NODAGS-Flow exhibits a decreasing trend in AUPRC score, while the DAG methods consistently score below the cyclic methods.  

\begin{figure}[ht]
    \centering
    \input{app-figures/varying-degree.tex}
    \caption{Performance comparison with varying latent graph sparsity.}
    \label{app-fig:varying-graph-sparsity}
\end{figure}

% \renewcommand{\arraystretch}{1.3}
% \setlength\tabcolsep{0.65em}
% \begin{table}[ht]
%     \centering 
%     \begin{tabular}{c|ccc|ccc}
%         \toprule
%         \multirow{2}{*}{\textbf{Sampler}} & \multicolumn{3}{c|}{\textbf{GAN}} & \multicolumn{3}{c}{\textbf{Linear Measurement}}\\ \cline{2-7}
%         & \textbf{AUPRC} & \textbf{SHD} & \textbf{Tr. Time} & \textbf{AUPRC} & \textbf{SHD} & \textbf{Tr. Time}\\   \hline\hline
%         SIR & 0.991 & 0.90 & 1.192 & 0.997 & 0.5 & 1.102\\
%         ULA & 0.993 & 1.30 & 3.389 & 0.954 & 3.10 & 3.267\\
%         Rejection & 0.977 & 2.25 & 11.256 & 0.997 & 0.5 & 8.27\\
%         \bottomrule
%     \end{tabular}    
% \end{table}
