# Supplementary material for: RECLAIM: Cyclic Causal Discovery Amid Measurement Noise
Source: arXiv:2603.20585 source file (2026-03-21)
Supplement: Supplementary file 3 [file em-convergence.tex]

\section{Convergence of EM algorithm}
\label{app:convergence}

Here, we provide the convergence analysis of RECLAIM's EM-based score maximization algorithm. Let $\mTheta^{(t)} = (\vtheta^{(t)}, \hat{\vphi})$. For ease of notation, we focus on a single interventional experiment $I_k \in \si$. However, the final result would still hold even when we consider the sum of likelihood over all the interventional experiments. Our analysis relies on the convergence of the EM algorithm \citep{wu_em_convergence,Friedman1998TheBS}, with the crux of it relying on establishing that the total log-likelihood of the observed variables either increases or stays the same in each iteration of the algorithm. That is, 
\begin{equation}\label{app-eq:m-step-requirement}
    \sum_{\ell=1}^{n_k} \log p(\vy^{(k, \ell)} \mid \mTheta^{t+1}, I_k) \geq \sum_{\ell=1}^{n_k} \log p(\vy^{(k, \ell)} \mid \mTheta^{t}, I_k)
\end{equation}

To that end, note that 
\begin{align*}
   \sum_{i=1}^{n_k} \log p(\vy^{(k, \ell)} \mid \mTheta, I_k) &= \sum_{i=1}^{n_k} \log p(\vy^{(k, \ell)}, \rvx^{(k, \ell)} \mid \mTheta, I_k) \\
    & \qquad - \sum_{i=1}^{n_k} \log p(\rvx^{(k, \ell)}\mid \vy^{(k, \ell)}, \mTheta, I_k)
\end{align*}
Taking expectation with respect $\rvx^{(k, \ell)}\mid \vy^{(k, \ell)}$ on both side, we get
\begin{align}
    \sum_{i=1}^{n_k} \log p(\vy^{(k, \ell)} \mid \mTheta, I_k) &=\sum_{i=1}^{n_k} \expect_{\rvx^{(k, \ell)}\mid \vy^{(k, \ell)}; \mTheta^{t}} \log p(\vy^{(k, \ell)} \mid \mTheta, I_k)\nonumber\\
    &= \underbrace{\sum_{i=1}^{n_k} \expect_{\rvx^{(k, \ell)}\mid \vy^{(k, \ell)}; \mTheta^{t}}\log p(\vy^{(k, \ell)}, \rvx^{(k, \ell)} \mid \mTheta, I_k)}_{= Q(\vtheta|\vtheta^t)}\nonumber\\
    & \quad -\sum_{i=1}^{n_k} \expect_{\rvx^{(k, \ell)}\mid \vy^{(k, \ell)}; \mTheta^{t}}\log p(\rvx^{(k, \ell)}\mid \vy^{(k, \ell)}, \mTheta, I_k).
    \label{app-eq:convergence-1}
\end{align}
The first term on the RHS in the above equation is nothing but $Q(\vtheta| \vtheta^t)$. This is maximized in the M-step, i.e., $Q(\vtheta| \vtheta^{t+1}) \geq Q(\vtheta| \vtheta^t)$. On the other hand, 
\begin{multline*}
\sum_{i=1}^{n_k} \expect_{\rvx^{(k, \ell)}\mid \vy^{(k, \ell)}; \mTheta^{t}}\log \frac{p(\rvx^{(k, \ell)}\mid \vy^{(k, \ell)}, \mTheta^{t+1}, I_k)}{p(\rvx^{(k, \ell)}\mid \vy^{(k, \ell)}, \mTheta^t, I_k)} = \\
 -D_{KL}\Big(p(\rvx^{(k, \ell)}\mid \vy^{(k, \ell)}, \mTheta^t, I_k)\big\|p(\rvx^{(k, \ell)}\mid \vy^{(k, \ell)}, \mTheta^{t+1}, I_k)\Big) \leq 0.
\end{multline*}
Thus, 
\begin{multline}
    \sum_{i=1}^{n_k} \expect_{\rvx^{(k, \ell)}\mid \vy^{(k, \ell)}; \mTheta^{t}}\log p(\rvx^{(k, \ell)}\mid \vy^{(k, \ell)}, \mTheta^{t+1}, I_k) \\ \leq \sum_{i=1}^{n_k} \expect_{\rvx^{(k, \ell)}\mid \vy^{(k, \ell)}; \mTheta^{t}}\log p(\rvx^{(k, \ell)}\mid \vy^{(k, \ell)}, \mTheta^t, I_k).
    \label{app-eq:convergence-2}
\end{multline}
From combining \cref{app-eq:convergence-1,app-eq:convergence-2}, we can see that at the end of the M-step \cref{app-eq:m-step-requirement} is satisfied. Thus, RECLAIM reaches a stationary point of the optimization objective.
