# Supplementary material for: RECLAIM: Cyclic Causal Discovery Amid Measurement Noise
Source: arXiv:2603.20585 source file (2026-03-21)
Supplement: Supplementary file 4 [file implementation-details.tex]

\section{Implementation Details}
\label{app:implementation-details}

In this section we provide further technical details on the implementation of RECLAIM and the baselines. 

\subsection{Projection Vector Sampling for Measurement Noise Estimation}
\label{app:projection-sampling}

The overall projection vector sampling algorithm for noise variance estimation is summarized in \cref{app-alg:projection-sampling}. We start with an empty $\mT_2$ matrix and iterating through each node in the latent graph. For each $i \in [d]$, let $\mM_i$ be the measurement matrix $\mA$ excluding the $i$-th column. We then compute its singular value decomposition (SVD) and extract the columns of $\mV$ matrix corresponding to zero singular values, denoted as $\mB_i$. These columns represent the basis vectors of the null space of $\mM_i$. A random vector $\vecu$ is then generated to obtain the projection matrix $\vt = \mB_i\vecu$. The vector $\vt$ is appended to $\mT_2$ if it provided sufficient signal and is sufficiently diverse from the existing projection vectors already in $\mT_2$. The process concludes once we sample the required number of rows for $\mT_2$. \Cref{theorem:full-rank-possible} guarantees that the above procedure would conclude and the results matrix $\mT_2$ would be full (column) rank. 

\begin{algorithm}[t]
\caption{Sampling Projection Vectors for Noise Estimation}
\label{app-alg:projection-sampling}
\begin{algorithmic}[1]
\Require Measurement matrix $\mA \in \R^{p \times d}$, intervention family $\si$ 
satisfying \cref{cond:channel-indentifiability-interventions}, thresholds 
$\epsilon_\text{sig} > 0$, $\delta > 0$, target number of vectors $m$
\Ensure Projection matrix $\mT_2 \in \R^{m \times p}$
\State Initialize $\mT_2 \leftarrow [\,]$
\For{$i = 1, \ldots, d$}
    \State Compute $\mM_i \leftarrow \mA_{-i}^\top \in \R^{(d-1) \times p}$
    \State Compute SVD: $\mM_i = \mU \mSigma \mV^\top$
    \State Extract basis $\mB_i \in \R^{p \times r}$ from columns of $\mV$ corresponding 
    to zero singular values, where $r = p - d + 1$
    \While{fewer than $\lfloor m/d \rfloor$ vectors collected for node $i$}
        \State Sample $\vecu \sim \mathcal{N}(\bm{0}, \mI_r)$
        \State Set $\vt \leftarrow \mB_i \vecu$
        \If{$|\veca_i^\top \vt| < \epsilon_\text{sig}$} \Comment{weak signal}
            \State \textbf{reject} and \textbf{continue}
        \EndIf
        \State Normalize: $\vt \leftarrow \vt / \|\vt\|$
        \If{$\exists\, (\vt^\prime)^{\odot} \in \mT_2$ s.t. $\cos\big(\vt^{\odot}, 
        (\vt^\prime)^{\odot}\big) > 1 - \delta$} \Comment{insufficient diversity}
            \State \textbf{reject} and \textbf{continue}
        \EndIf
        \State Append $(\vt^\odot)^\top$ to $\mT_2$
    \EndWhile
\EndFor
\State \Return $\mT_2$
\end{algorithmic}
\end{algorithm}

\subsection{Log-determinant of the Jacobian Computation}
\label{app:log-det-jacobian}

Computing the log-determinant of the Jacobian computation poses a significant challenge when evaluation the log-density of the latent variables. To overcome this issue, we exploit the power-series expansion of $\log(1 - x)$ to obtain the following: 
\begin{equation}
    \log \big|\det J_{(\id - \mU f)}(\rvx)\big| = 
    -\sum_{m=1}^\infty \frac{1}{m} \mathrm{Tr}\Big\{J^m_{\mU f}(\rvx)\Big\}.
    \label{app-eq:power-series}
\end{equation}
This brings the complexity of down to $\mathcal{O}(d^2)$. Further improvement can be made by using \emph{Hutchinson trace estimator}~\citep{hutchtraceestimator}
$$\mathrm{Tr}\Big\{J^m_{\mU f}(\rvx)\Big\} = \expect_{\mW}\Big[\mW^\top J^m_{\mU f}(\rvx)\mW\Big],$$
where $\mathbb{E}[\mW] = 0$ and $\mathbb{E}[\mW\mW^\top] = \mI$. The above estimator only depends on a vector-Jacobian product which can be efficiently computed using an auto-differentiation library (such as PyTorch), often reducing the complexity to $\mathcal{O}(d)$. In practice, the power series is truncated to a finite number of terms. This, however, introduces bias in the log-determinant of the Jacobian estimate. To improve on this, following~\cite{russianroulette}, the series cut-off $n$ is randomly sampled, $n \sim p_N$, where $p_N$ is a distribution over natural numbers $\mathbb{N}$. The individual terms in \cref{app-eq:power-series} are then reweighted by the inverse probability of ending there. Finally, we have the following unbiased estimator: 
\begin{equation}\label{app-eq:unbiased-log-det}
    \log \big|\det J_{(\id - \mU f)}(\rvx)\big| = 
    -\expect_{n, \mW} \Bigg[\sum_{m=1}^n \frac{\mW^\top J^m_{\mU f}(\rvx)\mW}{m\cdot P(N\geq n)} \Bigg].
\end{equation}

\subsection{RECLAIM and Baselines Code Details}

\paragraph{RECLAIM.} Our framework was built using the \texttt{Pytorch} library in Python and the code is provided as a part of the supplementary materials. 

We follow the setup of \cite{sethuraman2023nodags}, employing neural networks (NNs) with dependency masks parameterized by a Gumbel-softmax distribution. The log-determinant of the Jacobian is computed using a power series expansion combined with the Hutchinson trace estimator. To mitigate bias from truncating the power series expansion, the number of terms is sampled from a Poisson distribution, as detailed in \cref{sec:reclaim,app:log-det-jacobian}. The final objective is optimized using the Adam optimizer \citep{kingma2015adam}.

The learning rate in all our experiments was set to $10^{-2}$. The neural network models used in our experiments contained one multi-layer perceptron layer and \texttt{tanh} activation. The graph sparsity regularization constant $\lambda$ was set to $10^{-3}$ for all the experiments. The models were trained and evaluated on NVIDIA RTX6000 GPUs. 

\paragraph{Baselines. } For NODAGS-Flow, we used the code provided by authors \citep{sethuraman2023nodags} available at \url{https://github.com/Genentech/nodags-flows}. The default values were set for the hyperparameters. For DCDI, we used the codebase provided by the authors \citep{brouillard2020differentiable}, available at \url{https://github.com/slachapelle/dcdi}. The default hyperparameters were used while training and evaluating the model. For Anchored-CI, we implemented Algorithm 1 in~\citep{saeed2020anchored} using an implementation of PC algorithm available in \texttt{CausalDag} library in Python.
