# Supplementary material for: RECLAIM: Cyclic Causal Discovery Amid Measurement Noise
Source: arXiv:2603.20585 source file (2026-03-21)
Supplement: Supplementary file 5 [file solvability.tex]

\section{Solvability of Cyclic SCMs}
\label{sec:solution-to-sem}

Consider the cyclic SCM defined below: 
\begin{equation}\label{app-eq:scm}
    \rvx = f(\rvx) + \rvz. 
\end{equation}
% Need for function contractivity
In general, it is not guaranteed that \cref{app-eq:scm} has solution, this is primarily due to the (potential) presence of cycles in $\gr$. In order to see why this is true, note that, we can view \cref{app-eq:scm} as the unique fixed point (if it exists) to the following discrete time dynamical system:
\begin{equation}
    \label{app-eq:discrete-time-dynamical-system}
    \rvx(t+1) = f\big(\rvx(t)\big) + \rvz,
\end{equation}
where $\rvx(t)$ denotes the value of the random variable $\rvx$ at time $t$. In the following example, we illustrate how the choice of $f$ dictates whether or not \cref{app-eq:discrete-time-dynamical-system} attains a unique fixed point.

\begin{example}\label{example:no-fixed-point}
    Consider $X_1, X_2 \in \R$ given by the following structural equations:
    $$X_1(t+1) = aX_2(t) + Z_1, \quad X_2(t+1) = bX_1(t) + Z_2.$$
    \Cref{app-fig:example-no-fixed-point} shows an illustration of the evolution of trajectories for two different choices of the parameters $(a, b)$. From the right plot we can see that when we set $a=1.2$, and $b=2.3$, the systems is unstable and trajectory diverges. On the other hand, when $a=0.7$ and $b=-0.8$ (left plot), the system is stable and reaches a stationary point. 
\end{example}

To ensure \cref{app-eq:discrete-time-dynamical-system} admits a unique fixed point, we must impose additional restrictions on the causal mechanism $f$. One sufficient condition is to require $f$ to be \emph{contractive}.

\begin{definition}[Contractive function]
    A function $f : \R^d \to \R^d$ is said to be contractive if there exists a constant $L < 1$ such that for all $\vx, \vy \in \R^d$,
    $$\norm{f(\vx) - f(\vy)}_2 \leq L \norm{\vx - \vy}_2.$$
    The constant $L$ is called the Lipschitz constant. 
\end{definition}

When the causal mechanism $f$ is contractive, Banach fixed point theorem gaurantees that \cref{app-eq:discrete-time-dynamical-system} has a unique fixed point~\cite[theorem 9.23]{rudin2021principles}. Consequently, the causal mechanisms considered in this work are restricted to be contractive and neural networks are used to model the causal mechanism in practice. Contractivity is achieved via spectral scaling of the layer weights as described in \cref{sec:latent-likelihood} in the main paper. 

\begin{figure}[t]
\centering
\input{app-figures/example-no-fixed-point}
\caption{Illustration of state evolution for different choice of $a$ and $b$ for the system defined in \cref{example:no-fixed-point}. (Left) Choosing $a = 0.7$ and $b=-0.8$ results in a stable system and the system reaches a fixed point. (Right) Choosing $a = 1.2$ and $b = 2.3$ results in an unstable system and the trajectory diverges. }
\label{app-fig:example-no-fixed-point}
\end{figure}
