# Supplementary material for: RECLAIM: Cyclic Causal Discovery Amid Measurement Noise
Source: arXiv:2603.20585 source file (2026-03-21)
Supplement: Supplementary file 6 [file theoretical-considerations.tex]

\section{Proofs}
\label{app:theoretical-considerations}

All the proofs are contained in this section. Starting with proof of \cref{prop:projection-existence} in \cref{app:prop-projection-existence-proof}. \Cref{app:theorem-full-rank-possible-proof} contains the proof of \cref{theorem:full-rank-possible}. Finally, \cref{app:theorem-consistency-proof} contains the proof for \cref{theorem:consistency}. 

\subsection{Proof of \texorpdfstring{\Cref{prop:projection-existence}}{Proposition 3}}

\label{app:prop-projection-existence-proof}

\begin{proof}
    The claim of the proposition is equivalent to the following statement: 
    $$\mathcal{N}(\mA_{-i}^\top) \not\subset \veca_i^\perp.$$
    Since $\rank(\mA) = d$, the vector $\veca_i \notin \text{span}(\{\veca_j\}_{j\neq i})$ as the columns of $\mA$ are linearly independent. Furthermore, the null space of $\mA_{-i}^\top$ is the orthogonal complement of the span of the columns of $\mA_{-i}$, i.e., $\mathcal{N}(\mA_{-i}^\top) = \text{span}(\{\veca_j\}_{j\neq i})^\perp$. 

    Now, \emph{let us assume, for the sake of contradiction that} for each $\vt \in \R^p$ such that $\mA_{-i}^\top \vt = \bm{0}$, we have $\veca_i^\top \vt = 0$. This would mean that 
    $$\mathcal{N}(\mA_{-i}^\top) \subset \veca_i^\perp.$$ 
    Taking orthogonal complement on both sides, we get 
    $$(\veca_i^\perp)^\perp \subset \mathcal{N}(\mA_{-i}^\top)^\perp.$$ 
    Note that, $(\veca_i^\perp)^\perp = \spn(\veca_i)$, and also that $\mathcal{N}(\mA_{-i}^\top)^\perp = \spn(\{\veca_j\}_{j\neq i})$. That is,
    $\spn(\veca_i) \subset \spn(\{\veca_j\}_{j\neq i}).$
    This is a contradiction. Thus, there exists a vector $\vt \in \R^p$ such that $\veca_i^\top \vt \neq 0$ and $\mA_{-i}^\top \vt = \bm{0}$.  
\end{proof}

\subsection{Proof of \texorpdfstring{\Cref{theorem:full-rank-possible}}{Theorem 4}}
\label{app:theorem-full-rank-possible-proof}

Before we prove the theorem above, we state a technical lemma from functional analysis which is utilized in the proof of the theorem. 

\begin{lemma}\label{app-lemma:non-trivial-polynomials}
Let $P: \R^n \to \R$ be a non-trivial polynomial, then the zero set of $P$ has zero Lebesgue measure.     
\end{lemma}

See~\cite{folland1999real} for more details on \cref{app-lemma:non-trivial-polynomials}. We are now ready to prove \cref{theorem:full-rank-possible}

\begin{proof}[\Cref{theorem:full-rank-possible}]
    We divide the proof into two parts. In part 1, we show the existence of a measurement matrix $\mA_0$ that is not a part of $\bar{\mathcal{A}}$. Then, in part 2, using the result from part 1 we then conclude that the set $\bar{\mathcal{A}}$ has zero Lebesgue measure. 
    
    \vspace{0.3cm}
    \noindent
    \emph{Part 1: Existence of a measurement matrix $\mA_0$ such that $\mT_2$ is full rank}

    \vspace{0.3cm}
    \noindent
    For $p \geq d$, let us define $\mA_0$ as follows: 
    $$
    \mA_0 = \begin{bmatrix}
    \mI_d\\
    \mathbf{0}
    \end{bmatrix}, \quad \text{i.e., }\veca_{0,i} = \ve_i \text{ for } i = 1, \ldots, d. 
    $$
    For $i = 1, \ldots, d$, let $\vt^{(i)} = \ve_i$, and for $i = d+1, \ldots, p$, let $\vt^{(i)} = \ve_1 + \ve_i$. It is easy to check that $\{\vt^{(1)}, \ldots, \vt^{(p)}\} \subseteq \mathcal{T}(\mA_0)$. Thus, $\mT_2$ takes the following form: 
    $$
    \mT_2 = \begin{bmatrix}
    \mI_d & \mathbf{0}\\
    \mE_{1, p-d} & \mI_{p-d}\
    \end{bmatrix}
    $$
    where $\mE_{1, p-d} \in \R^{p-d \times d}$ denotes a matrix with ones in the first column and zeros everywhere else. Clearly, $\rank(\mT_2) = p$, i.e., $\mT_2$ is full rank. Thus, we have shown the existence of a non-trivial measurement matrix $\mA_0 \notin \bar{\mathcal{A}}$.  

    \vspace{1cm}
    \noindent
    \emph{Part 2: $\bar{\mathcal{A}}$ has zero Lebesgue measure}

    \vspace{0.3cm}
    \noindent
    Since $\rank(\mA) = d$, we know that $\rank(\mA_{-i}) = d-1$, and thus, $\mA_{-i}^\top \in \R^{(d-1) \times p}$ has rank $d-1$. Then, there exists a subset of rows $J_i \subset \{1, \ldots, p\}$, with $|J_i| = d-1$ such that the square matrix
    $$\mM_i(\mA) \triangleq (\mA_{-i})_{J_i, \ast} \in \R^{(d-1) \times (d-1)}$$
    is invertible. 

    Let $\vt$ be such that $\mA_{-i}^\top \vt = 0$ for some $i \in [d]$. Then, 
    $$\mM_i(\mA)^\top\vt_{J_i} + \mR_i(\mA)^\top\vt_{[p] \setminus J_i} = 0,$$
    where $\mR_i(\mA)$ denotes the submatrix of $\mA$ formed by rows not included in $J_i$. Since $\mM_i(\mA)$ is invertible, we have
    $$\vt_{J_i} = -\Big(\mM_i(\mA)^\top\Big)^{-1}\mR_i(\mA)^\top\vt_{[p] \setminus J_i}.$$
    Thus, every admissible $\vt$ has to have the following form: 
    $$
    \vt(\mA, \vecu) = \begin{bmatrix}
    -\Big(\mM_i(\mA)^\top\Big)^{-1}\mR_i(\mA)^\top\vecu\\
    \vecu
    \end{bmatrix}, \quad \vecu \in \R^{p-d}.
    $$
    Moreover, 
    $$\mM_i(\mA)^{-1} = \frac{\text{adj}(\mM_i(\mA))}{\det(\mM_i(\mA))}$$
    Thus, the each coordinate of $\vt(\mA, \vecu)$ are: linear in $\vecu$, divided $\det(\mM_i(\mA))$, and multiplied by polynomial functions of entries of $\mA$. Upon taking Hadamard product with itself, each entry of $\vt^\odot$ is a polynomial function of $\vecu$ and the entries of $\mA$ divided by the determinant of the minor matrices.

    Suppose we choose $p$ such vectors $\vt^{(1)}, \ldots, \vt^{(p)}$ (each possibly corresponding to different column of $\mA$). The determinant of the resulting $\mT_2$, $\det(\mT_2)$ is also polynomial in $\vecu^{(\ell)}$, for $\ell \in [p]$; and polynomial in entries of $\mA$  along with a division of the determinant of the minor matrices. That is, 
    $$\det(\mT_2) = \frac{\text{Polynomial in } \mA, \vecu^{(1)}, \ldots, \vecu^{(p)}}{\prod_{\ell=1}^p \det(\mM_\ell(\mA))^{k_\ell}}$$

    Let us define $$D(\mA) \triangleq \prod_{\ell=1}^p \det(\mM_\ell(\mA))^{k_\ell}$$ and $$P(\mA, \vecu^{(1)}, \ldots, \vecu^{(p)}) \triangleq D(\mA) \cdot \det(\mT_2). $$

    Note that, since the minor matrices are invertible 
    $$P(\mA, \vecu^{(1)}, \ldots, \vecu^{(p)}) = 0 \iff \det(\mT_2) = 0. $$

    In \emph{Part 1}, we showed the existence of an $\mA_0$ and $\vecu_0^{(1)}, \ldots, \vecu_0^{(p)}$ for which the function $P(\mA_0, \vecu_0^{(1)}, \ldots, \vecu_0^{(p)}) \neq 0$. Thus the polynomial $P$ is non-trivial. Hence, from \cref{app-lemma:non-trivial-polynomials}, the zero set of $P$ has zero Lebesgue measure. Thus, $\bar{\mathcal{A}}$---which is a subset of the zero set of $P$---has zero Lebesgue measure. 
\end{proof}

\subsection{Proof of \texorpdfstring{\Cref{theorem:consistency}}{Theorem 5}}

\label{app:theorem-consistency-proof}

In this subsection we provide the proof of consistency of RECLAIM under exact maximization. We start by reviewing the relevant definitions and prior results required to prove \cref{theorem:consistency}. 

\subsubsection{Preliminaries} 

Consider a directed graph $\gr = (\sx, \se)$. A \emph{path} $\pi$ between nodes $X_i$ and $X_k$ is a sequence of nodes $(X_{i_0}, X_{i_1}, \ldots, X_{i_n})$, with $X_{i_0} = X_i$, $X_{i_n} = X_k$, and every two consecutive nodes in the sequence are connected by an edge, i.e., either $X_{i_j} \to X_{i_{j+1}} \in \se$ or $X_{i_j} \gets X_{i_{j+1}} \in \se$ for all $j = 0, \ldots, n-1$, with $X$. A path is \emph{directed} if all the edges from $X_i$ to $X_k$ are oriented the same way. A cycle through node $X_i$ consists of a directed path from $X_i$ to a node $X_j$ and the directed edge $X_j \to X_i$. For a node $X_i$, the set of \emph{ancestors} is defined as $\text{an}_\gr(X_i) := \{X_j \in X \mid \text{a directed path exists between } X_j \text{ and } X_i\}$. Similarly, the \emph{descendant} of a node is defined as $\text{de}_\gr(X_i) := \{X_j \in X \mid \text{a directed path exists between } X_i \text{ and } X_j\}$. The \emph{strongly connected component} of a node $X_i$ is given by the intersection of the ancestors and the descendants of $X_i$, i.e., $\text{sc}_\gr(X_i) = \text{an}_\gr(X_i) \cap \text{de}_\gr(X_i)$. We can apply these definitions to subsets $\sx_U$ by taking the union over all the elements in the subset, i.e., $\text{de}_\gr(\sx_U) = \cup_{i \in U} \text{de}_\gr(X_i)$. Finally, a node $X_i$ is called a \emph{collider} in a path $\pi$ if it satisfies the following two conditions: (i) it is a non-endpoint node, and (ii) the subpath $(X_k, X_i, X_j)$ is of the form $X_k \to X_i \gets X_j$. 

In a cyclic graph, the notion of $\sigma$-separation was introduced by~\cite{forre2017markov} to relate structural properties in the graph to independencies observed in the generated distribution. 

\begin{definition}[$\sigma$-separation]
    Let $\gr = (\sx, \se)$ be a directed graph and let $\sx_C \subseteq \sx$ be a subset of nodes. A path $\pi = (X_{i_0}, X_{i_1}, \ldots, X_{i_n})$ is said to be $\sigma$-blocked given $\sx_C$ if 
     \begin{enumerate}
         \item the first node of $\pi$, $X_{i_0} \in \sx_C$ or its last node $X_{i_n} \in \sx_C$, or 
         \item $\pi$ contains a collider $X_j \notin \sx_C$,
         \item $\pi$ contains a non-collider $X_j \in \sx_C$ that points towards a neighbor that is not in the same strongly connected component as $X_j$ in $\gr$, i.e., $X_k \gets X_j \in \pi$ and $X_k \notin \text{sc}_\gr(X_j)$, or $X_j \to X_\ell \in \pi$ and $X_\ell \notin \text{sc}_\gr(X_j)$. 
    \end{enumerate}
     The path $\pi$ is said to be $\sigma$-open given $\sx_C$ if it is not $\sigma$-blocked. Two subsets of nodes $\sx_A, \sx_B \subseteq \sx$ is said to be $\sigma$-separated given $\sx_C$ if all the paths between $X_a$ and $X_b$, where $a \in A$ and $b \in B$, are $\sigma$-blocked given $\sx_C$, and is denoted by
     $$\sx_A \mathop{\perp}_{\gr}^{\sigma} \sx_B \mid \sx_C.$$
\end{definition}

When the graph is cyclic, $\sigma$-separation defined above reduces to the standard $d$-separation. We node define the property that connects $\sigma$-separations with distributional independencies. 

\begin{definition}[General directed global Markov Property~\citep{forre2017markov}]
    Let $\gr = (\sx, \se)$ be a directed graph and $p$ denote the probability density of the observations $\sx$. The probability density $p$ satisfies the \emph{general directed global Markov property} if for $\sx_A, \sx_B, \sx_C \subseteq \sx$
    $$\sx_A \mperp_\gr^\sigma \sx_B \mid \sx_C \implies \rvx_A \mperp_{p} \rvx_B \mid \rvx_C,$$
    where $\rvx_A \mperp_{p} \rvx_B \mid \rvx_C,$ denotes conditionally independence of $\rvx_A$ and $\rvx_B$ given $\rvx_C$ with respect to $p$. 
\end{definition}

\paragraph{Joint causal modeling of interventions.} We adopt the \emph{joint causal inference} (JCI) framework proposed by~\cite{mooij2020joint} to unify multiple interventional settings into a single representative system. This is done by augmenting the system with context variables $\sce_\si = (\rvc_1, \ldots, \rvc_K)$, where $\rvc_k$ corresponds to the $k$-th interventional setting $I_k$, we call this the \emph{meta system}. We consider the system to be under the $k$-th interventional setting when $\rvc_j = \emptyset$ for $j \neq k$ and $\rvc_k = \bm{\xi}_{I_k}$ where $\bm{\xi}_{I_k} \in \R^{|I_k|}$. Additionally, we construct an augmented graph $\gr^\si$ consisting of both the latent system variables $\sx$ and the context variables $\sce_\si$. The children of each context variable $\rvc_k$ are the interventional targets in $I_k$, i.e., $\text{ch}_{\gr^\si}(\rvc_k) = \sx_{I_k}$. Note that there are no edges going from variables in $\sx$ to the context variables $\sce_\si$, \seeref{app-fig:aug-graph}. Finally, given a family of interventional targets $\si = \{I_k\}_{k=1}^K$, and the corresponding context variables $\sce_\si$, the structural equations governing the meta system is given by   
\begin{equation*}
    \tilde{f}_i(\pa_{\gr^\si}(X_i), Z_i) = \begin{cases}
        (\rvc_k)_i & \text{if }, \exists k \in [K] \text{s.t. } \rvc_k \neq\emptyset, X_i \in \sx_{I_k},\\
        f_i(\pa_\gr(X_i)) + Z_i, & \text{otherwise}.\\
    \end{cases}
\end{equation*}
Note that $\pa_{\gr^\si}(X_i)$ includes both latent system variables and the context variables. The meta-SCM above defines a probability distribution over the joint meta-system variables: 
\begin{equation}\label{app-eq:meta-prob-density}
    p_{\gr^\si}(\rvx, \sce_\si) = p_{\gr^\si}(\sce_\si)p_{\gr^\si}(\rvx\mid\sce_\si),
\end{equation}
where $p_{\gr^\si}(\sce_\si)$ is called the \emph{context distribution} and as noted by~\cite{mooij2020joint}, the behavior of the system is unaffected by the context distribution. Furthermore, when $\rvc_k = \emptyset$ for all $k \in [K]$, $p_{\gr^\si}(\rvx\mid\sce_\si)$ becomes the observational data, and
$$
p_{\gr^\si}(\rvx \mid \rvc_k = \bm{\xi}_{I_k}, \rvc_{-k} = \emptyset) = p_{\tdo(I_k)(\gr)}(\rvx).
$$
Recall, for the interventional setting $I_k$, probability density governing the latents $\rvx$ is given by \cref{eq:prob-density-interventions} which we repeat here for convenience
\begin{equation*}
    p_{\tdo(I)(\gr)}(\rvx) = p_C(\rvx_I)p_Z\big(\rvz_{[d]\setminus I}\big)\big|J_{(\id - \mU f)}(\rvz)\big|.
\end{equation*}

\begin{figure}[t]
\centering 
\input{app-figures/augmented-graph}
\caption{Illustration of the augmented graph $\gr^\si$ corresponding the set of interventional targets $\si = \{\emptyset, \{1\}, \{3\}\}$. (b) and (c) represent the mutilated graph obtained after interventions on $X_1$ and $X_3$ respectively. The augmented graph is the union of $\gr$, $\tdo(\{X_1\})(\gr)$, and $\tdo(\{X_3\})(\gr)$ along with the context variables $C_1$ and $C_2$. } 
\label{app-fig:aug-graph}
\end{figure}

\begin{definition}
    Let $\gr = (\sx, \se)$ be a directed graph, and $\si = \{I_k\}_{k=1}^K$ be a family of interventional experiments. Let $\sm_\si(\gr)$ denote the set of positive densities $p_{\gr^\si} : \R^{2d} \to \R$ such that $p_{\gr^\si}$ is given by \cref{app-eq:meta-prob-density} for all $f:\R^{d} \to \R^d$, with $f_i(\rvx) = f_i({\pa_\gr}(X_i))$, such that the resulting forward map $(\id - f)$ is a diffeomorphism, for all $(\sigma_{Z, 1}^2, \ldots, \sigma_{Z,d}^2)$ such that $\rvz \sim \mathcal{N}\big(0, \text{Diag}(\sigma_{Z,1}^2, \ldots, \sigma_{Z,K}^2)\big)$.
\end{definition}

$\sm_\si(\gr)$ denotes the set of interventional density generated by $\gr^\si$. We now show that these densities satisfy the general directed global Markov property.

\begin{prop}\label{app-prop:general-markov-property}
    Let $\gr = (\sx, \se)$ be a directed graph, and $\si = \{I_k\}_{k=1}^K$ be a family of interventional experiments, let $p \in \sm_\si(\gr)$, then $p$ satisfies the general directed global Markov property relative to $\gr^\si$.
\end{prop}

\begin{proof}
    For a directed graph $\gr$ and a choice of $f : \R^{d} \to \R^d$ such that the forward map $(\id - f)$ is a diffeomorphism, the structural equations are uniquely solvable with respect to each strongly connected component of $\gr$. Moreover, since the addition of context variable doesn't introduce any cycles, from~\cite[Theorem A.21]{bongers2021foundations}, the distribution $p_{\gr^\si}$ is unique and it satisfies the general directed global Markov property. 
\end{proof}

Given a family of interventional experiments, we now define a notion of an equivalence class of directed (cyclic) graphs based on the set of distributions induced by them. 

\begin{definition}[$\si$-Markov Equivalence Class]
    Two directed graphs $\gr$ and $\gr^\prime$ are $\si$-Markov equivalent if and only if $\sm_\si(\gr) = \sm_\si(\gr^\prime)$, denoted as $\gr \equiv_\si \gr^\prime$. The set of all directed graphs that are $\si$-Markov equivalent to $\gr$ is the $\si$-Markov equivalence class of $\gr$, denoted as $\si$-MEC$(\gr)$. 
\end{definition}

\subsubsection{Proof of \texorpdfstring{\Cref{theorem:consistency}}{Theorem 5}} 

We now prove the main theoretical contribution of this work. Recall the score function defined in \cref{sec:reclaim-score}
\begin{equation*}
    \score_\si(\gr) \triangleq \sup_{\vtheta, \vphi} \sum_{k=1}^K \expect_{\rvy \sim p^{(k)}} 
    \log p(\rvy \mid \vtheta, \vphi, I_k) - \lambda|\gr|,
\end{equation*}
where  $p^{(k)}$ is the true data-generating distribution for \( \si = \{I_k\}_{k=1}^K \), and $(\vtheta, \vphi)$ represents the model parameters (latent SCM and measurement process). In the context of the meta system, the score function above is equivalent to the following score: 
\[
\score_\si(\gr) \triangleq \sup_{\vtheta, \vphi} \expect_{(\rvy, \rvc) \sim p_\si^\ast} \log p_{\gr^\si}(\rvy, \rvc \mid \vtheta, \vphi) - \lambda |\gr|,
\]
where $p_\si^\ast$ denotes the joint ground-truth distribution for the observed and the context variables, and $p_{\gr^\si}(\rvy, \rvc \mid \vtheta)$ is given by 
\begin{equation}\label{app-eq:obs-to-latent-map}
p_{\gr^\si}(\rvy, \rvc \mid \vtheta, \vphi) = \int_{\rvx} p(\rvy \mid \rvx, \vphi) p_{\gr^\si}(\rvx, \rvc \mid \vtheta)\,d\rvx.    
\end{equation}
Note that $p(\rvy \mid \rvx, \vphi)$ is defined by the measurement process $g(\rvx, \rve)$. 

We define \( \spe_\si(\gr) \) as the set of all distributions \( p_{\gr^\si}(\rvx, \rvc  \mid \vtheta)\) that can be expressed by the model specified by \cref{eq:sem-combined,eq:prob-density-interventions} in the main paper, and \cref{app-eq:meta-prob-density}. That is,
$\spe_\si(\gr) := \{p \mid \exists\,\vtheta \text{ s.t } p = p_{\gr^\si}(\cdot \mid \vtheta)\}$. Thus, it is clear that $\spe_\si(\gr) \subseteq \sm_\si(\gr)$. Similarly, we define the of observed distributions expressable by $\gr$, denoted as $\spe_{Y, \si}(\gr) = \{p \mid \exists (\vtheta, \vphi) \text{ s.t. } p = p_{\gr^\si}(\cdot \mid \vtheta, \vphi)\}$. In the following proposition we show that $\spe_{Y, \si}(\gr)$ is uniquely determined by a $p \in \spe_\si(\gr)$ when $\si$ satisfies \cref{cond:channel-indentifiability-interventions}.

\begin{prop}\label{app-prop:map-injectivity}
    Let $\si = \{I_k\}_{k=1}^K$ be a family of interventional experiments satisfying \cref{cond:channel-indentifiability-interventions}. Then for a fixed set of measurement parameters $\vphi$, under both Gaussian additive noise (GAN) measurement process and linear measurement system, the map $T: \spe_\si(\gr) \to \spe_{Y, \si}(\gr)$ given by \cref{app-eq:obs-to-latent-map} is injective. 
\end{prop}

\begin{proof}
    Under \cref{cond:channel-indentifiability-interventions}, the measurement noise variance is fully identifiable (\seeref{sec:measurement-system-estimate} for more details). For sake of simplicity, let us assume that the noise variances are equal (the conclusion even otherwise) and set to $\sigma^2$. Taking the characteristic functions of $Tp = Tp^\prime$ and dividing by the non-vanishing Gaussian factor $e^{-\sigma^2\norm{\bm{\xi}}^2/2}$ yields $\expect_p [e^{-i\bm{\xi}^\top h(\rvx)}] = \expect_{p^\prime} [e^{-i\bm{\xi}^\top h(\rvx)}]$ for all $\bm{\xi}$. Here, $f(\rvx) = \rvx$ for GAN system and $f(\rvx) = \mA\rvx$ for linear measurement system. Thus, from the uniqueness of the characteristic function~\citep{billingsley1995probability}, $f_\#p = f_\#p^\prime$. Since $f$ is injective, $p = p^\prime$. 
\end{proof}

\Cref{theorem:consistency} relies on the following set of assumptions. The first one ensures that the model is capable of representing the ground truth distribution. 

\begin{assume}[Sufficient Capacity] \label{app-assume:sufficient-capacity}
    The joint ground truth distribution $p_\si^\ast$ is such that $p_\si^\ast \in \spe_\si(\gr^\ast)$, where $\gr^\ast$ is the ground truth latent graph. 
\end{assume}

In other words, there exists a $\vtheta$ such that $p_\si^\ast = p_{\gr^\si}(\cdot \mid \vtheta)$. The second assumption generalizes the notion of faithfulness assumption to the interventional setting. 

\begin{assume}[$\si$-$\sigma$-faithfulness]\label{app-assume:faithfulness}
For any subset of nodes $A, B, D \subseteq \sx \cup \sce_\si$, and $I_k \in \si$
$$A \mathop{\not\perp}_{\gr^\si}^\sigma B \mid D \implies \bm{A} \mathop{\not\perp}_{p_{\gr^\si}} \bm{B} \mid \bm{C}. $$
\end{assume}

The above assumption implies that any conditional independency observed in the data must imply a $\sigma$-separation in the corresponding interventional ground truth graph. 

\begin{assume}[Strict positivity]\label{app-assume:positivity}
    For all $(\rvx, \rvc)$ and $p_{\gr^\si} \in \sm_\si(\gr)$, $p_{\gr^\si}(\rvx, \rvc) > 0$. 
\end{assume}

\begin{assume}[Finite differential entropy]\label{app-assume:finite-entropy}
    For a family of interventions $\{X_{\si_m}\}_{m=0}^M$,
    $$ \abs{ \expect_{p_\si^\ast}\log p_\si^\ast(\rvy, \rvc) } < \infty.$$
\end{assume}

The last two assumptions ensure that the scenario where $\score(\gr^\ast)$ and $\score(\gr)$ are both infinity is avoided. This is formalized in the lemma below taken from~\cite{brouillard2020differentiable}. 

\begin{lemma}[Finiteness of the score function \citep{brouillard2020differentiable}]
    Under the \cref{app-assume:sufficient-capacity,app-assume:finite-entropy}, the score function is finite, that is, $|\score_\si(\gr)| < \infty$. 
\end{lemma}

We finally make the assumption that the parameter space of $\vtheta$ and $\vphi$ are compact. 

\begin{assume}[Parameter compactness]\label{app-assume:parameter-compactness}
    The parameters of the measurement process $\vphi$ belong to a compact metric space $\Phi$.  
\end{assume}

For the both Gaussian additive noise (GAN) and linear measurement system, the parameters correspond to the variance of the Gaussian distribution, $\vphi = (\sigma_1^2, \ldots, \sigma_p^2)$. For the case of GAN system, $p = d$. The implication of the above assumption is that $\sigma_j^2 \leq \sigma_{\max}^2$, i.e., it is bounded above. Additionally, note that since we restrict the causal mechanism to \emph{contractive}, the parameters of latent SCM also belong to a compact space. 

From the results of~\cite{brouillard2020differentiable}, we can now express the difference in score function between $\gr^\ast$ and $\gr$ as the minimization of KL diverengence plus the difference in the regularization terms. 

\begin{lemma}[Rewritting the score function \citep{brouillard2020differentiable}]\label{app-lemma:scores}
    Under assumptions \ref{app-assume:sufficient-capacity} and \ref{app-assume:finite-entropy}, we have 
    $$\score(\gr^\ast) - \score(\gr) = \inf_{\vtheta, \vphi} D_{KL}(p_{\si}^\ast\| p_{\gr^\si}(\cdot \mid \vtheta, \vphi)) + \lambda (|\gr| - |\gr^\ast|).$$
\end{lemma}

Furthermore, \cite{sethuraman2025differentiable} showed that the KL divergence appearing the in lemma above is strictly positive when the latent variables are directly observed. 

\begin{lemma}[Lemma A.18 \citep{sethuraman2025differentiable}]\label{app-lemma:strictly-pos}
    Let $\gr = (\sx, \se)$ be a directed graph, for a set of interventional targets $\si = \{I_k\}_{k=1}^K$, and $p^\ast \notin \sm_\si(\gr)$, then
    $$\inf_{p\in \sm_\si(\gr)} D(p^\ast\|p) > 0.$$
\end{lemma}

We now extend this result to the case of indirect measurements. 

\begin{lemma}\label{app-lemma:strictly-pos-obs}
    Let $\gr = (\sx, \se)$ be a directed graph, for a set of interventional targets $\si = \{I_k\}_{k=1}^K$ satisfying \cref{cond:channel-indentifiability-interventions}, and $p^\ast_Y \notin \sm_{Y,\si}(\gr)$, then
    $$\inf_{p\in \sm_{Y, \si}(\gr_m)} D(p^\ast_Y\|p_Y) > 0.$$
\end{lemma}

\begin{proof}
Since $\si$ satisfies \cref{cond:channel-indentifiability-interventions}, the parameters of the measurement process is fully identified. Moreover, from \cref{app-prop:map-injectivity}, the map $T: \spe_\si(\gr) \to \spe_{Y, \si}(\gr)$. Thus, $T^{-1}p_Y^\ast \notin \spe_\si(\gr)$. Thus, from \cref{app-lemma:strictly-pos}, no sequence $\{p^{(k)}\}_{k=1}^\infty \subset \sm_si(\gr)$ exists such that the limit $\lim_{k\to\infty} p^{(k)} = T^{-1}p_Y^\ast$. Therefore, there exists no sequence $\{p_Y^{(k)}\}_{k=1}^\infty \subset \sm_{Y,si}(\gr)$ such that $\lim_{k\to\infty} p_Y^{(k)} = p_Y^\ast$. Thus,
$$\inf_{p\in \sm_{Y, \si}(\gr_m)} D(p^\ast_Y\|p_Y) > 0. $$
This proves the lemma.
\end{proof}

We are now ready to prove \cref{theorem:consistency}. Recall,

\begin{customthm}{\ref{theorem:consistency}.}
    Let $\si = \{I_k\}_{k=1}^K$ be a family of interventional targets satifying \cref{cond:channel-indentifiability-interventions}, let $\gr^\ast$ denote the ground truth directed graph, $p^{(k)}$ denote the data generating distribution for $I_k \in \si$, and $\hat{\gr} := \arg\max_{\gr} \score(\gr)$. Then, under \cref{app-assume:sufficient-capacity,app-assume:faithfulness,app-assume:positivity,app-assume:finite-entropy,app-assume:parameter-compactness}, and for a suitably chosen $\lambda > 0$, we have that $\hat{\gr} \equiv_\si \gr^\ast$. That is, $\hat{\gr}$ is $\si$-Markov equivalent to $\gr^\ast$.
\end{customthm}

\begin{proof}
The proof is a direct extension of Theorem 2 in \cite{sethuraman2025differentiable}, with \cref{app-lemma:strictly-pos-obs} substituting \cref{app-lemma:strictly-pos}. Which we present here for self-containment. 

It is sufficient to show that for $\gr \notin \si\text{-MEC}(\gr^\ast)$, the score function of $\gr$ is strictly lower than the score function of $\gr^\ast$, i.e., $\score(\gr^\ast) > \score(\gr)$. Since \( \gr \notin \si\text{-MEC}(\gr^\ast) \) and \( p_\si^\ast\in \sm_\si(\gr^\ast) \) (by \cref{app-assume:sufficient-capacity}), there must exist subsets of nodes \( A, B, D \subseteq \sx \cup \sce_\si \) such that either:
\begin{equation}\label{eq:condition-1}
A \mperp_{\gr}^\sigma B \mid D \quad \text{and} \quad A \mathop{\not\perp}_{\gr^\ast}^\sigma B \mid D, \tag{C1}
\end{equation}
or
\begin{equation}\label{eq:condition-2}
A \mathop{\not\perp}_{\gr}^\sigma B \mid D \quad \text{and} \quad A \mperp_{\gr^\ast}^\sigma B \mid D, \tag{C2}   
\end{equation}
If no such subsets exist, then \( \gr \) and \( \gr^\ast \) impose the same  $\sigma$ -separation constraints and thus induce the same set of distributions. This would imply that \( \gr \in \si\text{-MEC}(\gr^\ast) \), contradicting our assumption. Since $p_\si^\ast \in \sm_\si(\gr^\ast)$, in the case of \eqref{eq:condition-1}, it must be true that $\bm{A} \not\perp_{p_\si^\ast} \bm{B} \mid \bm{D}$ (\cref{app-assume:faithfulness}). Therefore $p_\si^\ast$ doesn't satisfy the general directed Markov property with respect to $\gr^\si$ and hence $p_\si^\ast \notin \sm_\si(\gr)$. For \eqref{eq:condition-2}, if $p_\si^\ast \in \sm_\si(\gr)$, then from \cref{app-assume:faithfulness}, it must be true that $\bm{A} \not\perp_{p_\si^\ast} \bm{B} \mid \bm{C}$. However, $p_\si^\ast \in \sm_\si(\gr^\ast)$, and \cref{app-prop:general-markov-property} implies that $\bm{A} \perp_{p_\si^\ast} \bm{B} \mid \bm{C}$, resulting in a contradiction. Therefore, $p_\si^\ast \notin \sm_\si(\gr)$. Morevover, from \cref{app-prop:map-injectivity} we can conclude that $p_{Y, \si}^\ast \notin \sm_{Y, \si}(\gr)$.  

For convenience, let $$\eta(\gr) := \inf_{\vtheta} D_{KL}(p_{Y,\si}^\ast\|p_{Y, \gr^\si}(\cdot \mid \vtheta, \vphi^\ast)).$$
Note that
$$\eta(\gr) = \inf_{\vtheta} D_{KL}(p_{Y,\si}^\ast\|p_{Y, \gr^\si}(\cdot \mid \vtheta, \vphi^\ast)) \geq \inf_{p \in \sm_{Y,\si}(\gr)} D_{KL}(p_Y^{(k)}\|p_Y) > 0,$$
where we use \cref{app-lemma:strictly-pos-obs} for the final inequality. Thus, from Lemma~\ref{app-lemma:scores}
\begin{equation*}
    \score(\gr^\ast) - \score(\gr) = \eta(\gr) + \lambda(|\gr| - |\gr^\ast|).
\end{equation*}
Following \cite{brouillard2020differentiable}, we now show that by choosing $\lambda$ sufficiently small, the above equation is stictly positive. Note that if $|\gr| \geq |\gr^\ast|$ then $\score(\gr^\ast) - \score(\gr) > 0$. Let $\mathbb{G}^+ := \{\gr \mid |\gr| < |\gr^\ast|\}$. Choosing $\lambda$ such that $0 < \lambda < \min_{\gr \in \mathbb{G}^+} \frac{\eta(\gr)}{|\gr^\ast| - |\gr|}$ we see that: 
\begin{align*}
    &\lambda < \min_{\gr \in \mathbb{G}^+} \frac{\eta(\gr)}{|\gr^\ast| - |\gr|}\\
    \iff &\lambda < \frac{\eta(\gr)}{|\gr^\ast| - |\gr|} \quad \forall \gr \in \mathbb{G}^+\\
    \iff &\lambda (|\gr^\ast| - |\gr|) < \eta(\gr) \quad \forall \gr \in \mathbb{G}^+\\
    \iff & 0 < \eta(\gr) + \lambda(|\gr| - |\gr^\ast|) = \score(\gr^\ast) - \score(\gr) \quad \forall \gr \in \mathbb{G}^+.
\end{align*}
Thus, every graph outside of the general directed Markov equivalence class of $(\gr^\ast)^\si$ has a strictly lower score. 
\end{proof}
